# Supplementary material for: Regret and Belief Complexity Trade-off in Gaussian Process Bandits via Information Thresholding
Source: arXiv:2003.10550 source file (2022-03-21)
Supplement: Supplementary file 2 [file appendix_backup.tex]

\clearpage
\section*{\centering Supplementary Material}


%%%%%%%%%%%%%%%%%%%%%%%%%%%%%%%%%%%%%%%%%%%%%%%%%%%%%%%%%%%%%%%%%%%%%%%%%%%%%%%%%%%%%%%%%%%%%%%%%%%%%%%%%%%%%%%%%%%%%%%%%%%%%%%%%%%%%%%%%%%%%%%%%%%L E M M A%%%%%%%%%%%%%%%%%%%%%%%%%%%%%%%%%%%%
%%%%%%%%%%%%%%%%%%%%%%%%%%%%%%%%%%%%%%%%%%%%%%%%%%%%%%%%%%%%%%%%%%%%%%%%%%%%%%%%%%%%%%%%%%%%%%%%%%%%%%%%%%%%%%%%%%%%%%%%%%%%%%%%%%%%%%%%%%
\begin{lemma}\label{lemma1}
%
	Choose $\delta \in (0,1)$ and let $\beta_{t} = 2\log(|\mathcal{A}|\pi_{t}/\delta)$, for some $\pi_{t}$ such that $\sum_{t\geq 1} \pi_{t}^{-1} = 1, \pi_{t} >0$. Then
	%
	\begin{align}\label{eq:lemma1}
	%
	|f(\bbx)-\hat{\mu}_{t-1}(\bbx)| \leq {\beta}_{t}^{1/2}\hat{\sigma}_{t-1}(\bbx)\hspace{0.1in} \forall \bbx \in \mathcal{A}, \forall t \geq 1
	%
	\end{align}
	%
	holds with probability $\geq 1-\delta$.
	%
	\end{lemma}
	%
	%%%%%%%%%%%%%%%%%%%%%%%%%%%%%%%%%%%%%%%%%%%%%%%%%%%%%%%%%%%%%%%%%%%%%%%%%%%%%%%%%%%%%%%%%%%%%%%%%%%%%%%%%%%%%%%%%%%%%%%%%%%%%%%%%%%%%%%%%%%%%%%%%%% P  R  O  O  F%%%%%%%%%%%%%%%%%%%%%%%%%%%%%%%%%%%%%%%%%%%%%%%%
%%%%%%%%%%%%%%%%%%%%%%%%%%%%%%%%%%%%%%%%%%%%%%%%%%%%%%%%%%%%%%%%%%%%%%%%%%%%%%%%%%%%%%%%%%%%%%%%%%%%%%%%%%%%%%%%%%%%%%%%%%%%%%%%%%%%%%%%%%
	\begin{proof}
At each $t$, we have dictionary $\bbD_{t-1}$ which contains the data points for the function $f(\bbx)$. For a given $\bbD_{t-1}$, we  have $f(\bbx) \sim {N}(\hat{\mu}_{t-1},\hat{\sigma}_{t-1})$. Note that in the normal GP-UCB algorithm, since we are using compression at each time instant, we end up taking actions $\hat\bbx_{i=1:t}$ and observations $\hat y_{i=1:t}$ which are different from $\bbx_{i=1:t}$ and $y_{i=1:t}$ of the GP-UCB algorithm.  Hence, $(\hat{\mu}_{t-1},\hat{\sigma}_{t-1})$ defines a Gaussian distribution $\hat{\mathcal{G}}_{t-1}$ which is parametrized by the collection of data points $(\hat\bbx,\hat y)\in\bbD_{t-1}$. At $t$, we  take an action $(\hat \bbx_t)$ and observe $\hat y_t$. Then, we perform the update to obtain $(
\tilde{\mu}_{t-1},\tilde{\sigma}_{t-1})$ which defines the distribution $\tilde{\mathcal{G}}_t$. Next, we compress it such that $d_H(\hat{\mathcal{G}}_t,\tilde{\mathcal{G}}_t)\leq \epsilon$ where $\epsilon$ is the compression budget. Hence, there is a fundamental difference between both the algorithms and we seek to analyze the performance of the proposed algorithm in terms the regret defined against the optimal $f(\bbx^\star)$. For a random variable $r \sim N(0,1)$, the cumulative density function can be used to express
%
\begin{align}\label{eq:gaussian_tail_integration}
%
P(r>c) &= \frac{1}{\sqrt{2\pi}}\int_{c}^{\infty}e^{-\frac{r^2}{2}}dr\\
%
 &= e^{\frac{-c^2}{2}}\frac{1}{\sqrt{2\pi}}\int_{c}^{\infty}e^{((\frac{-r^2}{2}+rc-\frac{c^2}{2})+(-rc-c^2))}dr \nonumber \\
%
&=e^{-\frac{c^2}{2}}\frac{1}{\sqrt{2\pi}}\int_{c}^{\infty}e^{-\frac{(r-c)^2}{2}}e^{-c(r-c)}dr. \nonumber
%
\end{align}
%
For $c > 0$ and $r\geq c$, we have that $e^{-c(r-c)}\leq 1$. Furthermore, the integral term scaled by $\frac{1}{\sqrt{2\pi}}$ resembles the Gaussian density integrated from $c$ to $\infty$ for a random variable $r$ with mean $c$ and unit standard deviation, integrated to $1/2$. Therefore, we get
%
\begin{align}\label{eq:gaussian_tail_approximation}
%
P(r>c) \leq e^{-c^{2}/2} P(r>0)=\frac{1}{2}e^{-c^{2}/2}.
%
\end{align}
%
Using the expression $r = (f(\bbx)-\hat{\mu}_{t-1}(\bbx))/\hat{\sigma}_{t-1}(\bbx)$  and $c = \beta_{t}^{1/2}$ for some sequence of nonnegative scalars $\{\beta_t\}_{t\geq 0}$ {substituted into the left-hand side of \eqref{eq:gaussian_tail_integration} using the left-hand side of \eqref{eq:gaussian_tail_approximation} }, we obtain
%
\begin{align}
%
P\Big\{|f(\bbx)-\hat{\mu}_{t-1}(\bbx)|&>\beta_{t}^{1/2}\hat{\sigma}_{t-1}(\bbx)\Big\}\leq e^{-\beta_{t}/2}.
%
\end{align}
%
Now apply Boole's inequality to the preceding expression to write
%
\begin{align}
%
P\Big\{{{\bigcup}}_{\bbx \in \mathcal{A}}& |f(\bbx)-\hat{\mu}_{t-1}(\bbx)|>\beta_{t}^{1/2}\hat{\sigma}_{t-1}(\bbx)\Big\}\nonumber
\\
&\leq \sum_{\bbx \in \mathcal{A}} P\Big\{|f(\bbx)-\hat{\mu}_{t-1}(\bbx)|>\beta_{t}^{1/2}\hat{\sigma}_{t-1}(\bbx)\Big\}\nonumber
\\
&\leq |\mathcal{A}|e^{-\beta_{t}/2}.
%
\end{align}
%
To obtain the result in the statement of Lemma \ref{lemma1}, select the constant sequence $\beta_t$ such that $|\mathcal{A}|e^{\beta_{t}/2}=\frac{\delta}{\pi_{t}}$, with scalar parameter sequence $\pi_{t} := \pi^{2}t^{2}/6$. Applying the union bound again over all time points $t \in \mathbb{N}$, we get 
%
\begin{align}
% 
P\Big\{\bigcup_{t=1}^{\infty}& |f(\bbx)-\hat{\mu}_{t-1}(\bbx)|>\beta_{t}^{1/2}\hat{\sigma}_{t-1}(\bbx)\Big\}\nonumber
\\
\leq& \sum_{t=1}^{\infty} P\Big\{|f(\bbx)-\hat{\mu}_{t-1}(\bbx)|>\beta_{t}^{1/2}\hat{\sigma}_{t-1}(\bbx)\Big\}\nonumber\\
\leq& \sum^{\infty}_{t=1}\frac{\delta}{\pi_{t}}\nonumber\\ 
=& \delta.
%
\end{align}
%
The last equality $\sum^{\infty}_{t=1}\frac{\delta}{\pi_{t}} = \delta$ is true since $\sum^{\infty}_{t=1}1/t^{2} = \pi^{2}/6$. 
We can now change the inequality to obtain an upper bound on the absolute difference between the true function and the estimated mean function for all $\bbx \in \mathcal{A}$ and $t \geq 1$ such that
\begin{align}
%
	|f(\bbx)-\hat{\mu}_{t-1}(\bbx)| \leq {\beta}_{t}^{1/2}\hat{\sigma}_{t-1}(\bbx),\hspace{0.1in} \forall \bbx \in \mathcal{A}, \ \forall t \geq 1
	%
\end{align}
holds with probability $1-\delta$. This completes the proof.
	\end{proof}
%%%%%%%%%%%%%%%%%%%%%%%%%%%%%%%%%%%%%%%%%%%%%%%%%%%%%%%%%%%%%%%%%%%%%%%%%%%%%%%%%%%%%%%%%%%%%%%%%%%%%%%%%%%%%%%%%%%%%%%%%%%%%%%%%%%%%%%%%%%%%%%%%%%%L E M M A%%%%%%%%%%%%%%%%%%%%%%%%%%%%%%%%%%%%
%%%%%%%%%%%%%%%%%%%%%%%%%%%%%%%%%%%%%%%%%%%%%%%%%%%%%%%%%%%%%%%%%%%%%%%%%%%%%%%%%%%%%%%%%%%%%%%%%%%%%%%%%%%%%%%%%%%%%%%%%%%%%%%%%%%%%%%%%%

\begin{lemma}\label{lemma2}
%
	Fix $t \geq 1$. If 	$|f(\bbx)-\hat{\mu}_{t-1}(\bbx)| \leq \beta_{t}^{1/2}\hat{\sigma}_{t-1}(\bbx)$ for all $\bbx \in D$, the instantaneous regret is bound as
	%
	\begin{align}\label{eq:lemma2}
	%
	r_{t} \leq 2\beta_{t}^{1/2}\hat{\sigma}_{t-1}(\bbx_{t})
	%
	\end{align}
	%
\end{lemma}
%
	%%%%%%%%%%%%%%%%%%%%%%%%%%%%%%%%%%%%%%%%%%%%%%%%%%%%%%%%%%%%%%%%%%%%%%%%%%%%%%%%%%%%%%%%%%%%%%%%%%%%%%%%%%%%%%%%%%%%%%%%%%%%%%%%%%%%%%%%%%%%%%%%%%% P  R  O  O  F%%%%%%%%%%%%%%%%%%%%%%%%%%%%%%%%%%%%%%%%%%%%%%%%
%%%%%%%%%%%%%%%%%%%%%%%%%%%%%%%%%%%%%%%%%%%%%%%%%%%%%%%%%%%%%%%%%%%%%%%%%%%%%%%%%%%%%%%%%%%%%%%%%%%%%%%%%%%%%%%%%%%%%%%%%%%%%%%%%%%%%%%%%%
	\begin{proof}
Since the GP-UCB algorithm chooses the next sampling point $\bbx_{t}$ as the argmax of $\hat{\mu}_{t-1}(\bbx)+\sqrt{\beta_{t}}\hat{\sigma}_{t-1}(\bbx)$ at each step, we have
%
 \begin{align}
  \hat{\mu}_{t-1}(\hat\bbx_{t})+\sqrt{\beta_{t}}\hat{\sigma}_{t}(\hat\bbx_{t}) &\geq  \hat{\mu}_{t-1}(\bbx^{\star})+\sqrt{\beta_{t}}\hat{\sigma}_{t-1}(\bbx^{\star})\nonumber 
  \\
   &\geq f(\bbx^{\star}),
 \end{align} 
 %
 where $\bbx^{\star}$ is the optimal point. The instantaneous regret is then bounded as
 %
\begin{align}
%
r_{t} =& f(\bbx^{\star})-f(\hat\bbx_{t}) \nonumber 
\\
\leq&  \hat{\mu}_{t-1}(\hat\bbx)+\beta^{1/2}_{t}\hat{\sigma}_{t-1}(\hat\bbx_{t})-f(\hat\bbx_{t}).
%
\end{align}
%
But from Lemma \ref{lemma1} we have that $|f(\bbx)-\hat{\mu}_{t-1}(\bbx)| \leq \beta_{t}^{1/2}\hat{\sigma}_{t-1}(\bbx)$ holds with probability $1-\delta$. This implies that 
%\blue{This statement should only hold with high probability. Please clarify. Also what is $1(x^*)$?}, thus we obtain
%%
\begin{align}\label{regret1}
%
r_{t} = f(\bbx^{\star})-f(\hat\bbx_{t}) \leq  2\sqrt{\beta_{t}}\hat{\sigma}_{t-1}(\hat\bbx_{t}).
%
\end{align}
%
The expression in \eqref{regret1} represents the regret at instant $t$ for action $\hat{\bbx}_t$ taken by the proposed algorithm. 
\end{proof}
%%%%%%%%%%%%%%%%%%%%%%%%%%%%%%%%%%%%%%%%%%%%%%%%%%%%%%%%%%%%%%%%%%%%%%%%%%%%%%%%%%%%%%%%%%%%%%%%%%%%%%%%%%%%%%%%%%%%%%%%%%%%%%%%%%%%%%%%%%%%%%%%%%%%L E M M A%%%%%%%%%%%%%%%%%%%%%%%%%%%%%%%%%%%%
%%%%%%%%%%%%%%%%%%%%%%%%%%%%%%%%%%%%%%%%%%%%%%%%%%%%%%%%%%%%%%%%%%%%%%%%%%%%%%%%%%%%%%%%%%%%%%%%%%%%%%%%%%%%%%%%%%%%%%%%%%%%%%%%%%%%%%%%%%
\begin{lemma}\label{lemma3}
%
	The information gain for the points selected can be expressed in terms of the predicted variances. If $\bbf_T=(f(\hat\bbx_t))\in\mathbb{R}^T$:
	%
	\begin{align}
	%
I(\hat\bby_{T};\hat\bbf_{T})=& 
\frac{1}{2} \sum_{t\in M_T(\epsilon)}\log(1+\sigma^{-2}\hat{\sigma}^{2}_{t-1}(\bbx_{t}))
%
	\end{align}
	where $M_T(\epsilon)$ denotes the number of elements in the dictionary $\bbD_T$ and note that $M_T(0)=T$.
	%
\end{lemma}
%
	%%%%%%%%%%%%%%%%%%%%%%%%%%%%%%%%%%%%%%%%%%%%%%%%%%%%%%%%%%%%%%%%%%%%%%%%%%%%%%%%%%%%%%%%%%%%%%%%%%%%%%%%%%%%%%%%%%%%%%%%%%%%%%%%%%%%%%%%%%%%%%%%%%% P  R  O  O  F%%%%%%%%%%%%%%%%%%%%%%%%%%%%%%%%%%%%%%%%%%%%%%%%
%%%%%%%%%%%%%%%%%%%%%%%%%%%%%%%%%%%%%%%%%%%%%%%%%%%%%%%%%%%%%%%%%%%%%%%%%%%%%%%%%%%%%%%%%%%%%%%%%%%%%%%%%%%%%%%%%%%%%%%%%%%%%%%%%%%%%%%%%%
	\begin{proof}
	%
We remark that for the standard GP-UCB algorithm, at each iteration $t$, we have $\bby_t=[y_1, y_2, \cdots, y_t]^T$ which collects all the observations till $t$, and correspondingly in dictionary, we store $\bbX_t=[\bbx_1, \bbx_2, \cdots, \bbx_t]$ which collects all the actions takes so far. But for the compressed CGP-UCB algorithm, since we are only selecting a subset of the elements from $\hat{\bby}_t :=\{\hat y_{i}\}\in \bbD_t$ and $|\bbD_t| \leq t$ for all $t$ due to the $\epsilon$ compression at each step. For a Gaussian with covariance matrix $\sigma^{2}\bbI$, the information gain is~\citep{cover2012elements} is given by 
%
\begin{align}\label{information}
%
	I(\bby_{t};\bbf_{t}) = \mathbf{H}(\bby_{t})-\frac{1}{2}\log|2\pi e\sigma^{2}\bbI|,
	%
\end{align}
where it holds that
\begin{align}\label{first0}
%
\frac{1}{2}\log|2\pi e\sigma^{2}\bbI| = \frac{1}{2}\sum^{T}_{t=1}\log(2\pi e\sigma^{2})
%
\end{align}
% In a similar way, we can write 
Since $\bby_t\in\mathbb{R}^t$. In contrast, for the proposed CGP-UCB algorithm, we have $\hat\bby_t\in\mathbb{R}^{M_t}$ where $M_t(\epsilon)=|\bbD_t|$ represents the model order of the system. %
%\begin{align}
%%
%	I(\hat\bby_{t};\hat\bbf_{t}) = \mathbf{H}(\hat \bby_{t})-\frac{1}{2}\log|2\pi e\sigma^{2}\bbI|,
%	%
%\end{align}
%where it holds that
%\begin{align}\label{first}
%%
%\frac{1}{2}\log|2\pi e\sigma^{2}\bbI| = \frac{1}{2}\sum^{|\bbD_t|}_{t=1}\log(2\pi e\sigma^{2}).
%%
%\end{align}
%
Next, by expanding the entropy term $\mathbf{H}(\tilde\bby_{t})$ where $\tilde\bby_{t}=[\hat\bby_{t-1}; \hat y_{t}]$ before the compression,  we can write
%
\begin{align}\label{second}
%
%
\mathbf{H}(\hat\bby_{t}) 
&= \mathbf{H}(\hat\bby_{t-1})+\mathbf{H}(y_{t}|\hat\bby_{t-1}) 
\\
&= \mathbf{H}(\hat\bby_{t-1})+\frac{1}{2}\log\big(2\pi e(\sigma^{2}+\hat{\sigma}^{2}_{t-1}(\hat\bbx_{t}))\big). \nonumber
%
%&= \frac{1}{2}\sum^{T}_{t=1}\log(2\pi e\sigma^{2})+\frac{1}{2} \sum^{T}_{t=1}\log(1+\sigma^{-2}\hat{\sigma}^{2}_{t-1}(\bbx_{T})).\nonumber
%
%
\end{align}
We add the current information $\mathbf{H}(y_{t}|\hat\bby_{t-1})$ only if it is more than $\epsilon$ other other wise we don't. This also implies that we drop the update if $|\mathbf{H}(\hat\bby_{t})- \mathbf{H}(\hat\bby_{t-1})| \leq \epsilon$. The above expression holds for each $t$, now take summation over $t=1$ to $T$, since $\bbH(\hat\bby_0)=0$, we get 
\begin{align}\label{third}
%
%
\mathbf{H}(\hat\bby_{T}) 
=& \frac{1}{2}\sum_{t\in M_T(\epsilon)}\log(2\pi e\sigma^{2})\nonumber
\\
&+\frac{1}{2} \sum_{t\in M_T(\epsilon)}\log(1+\sigma^{-2}\hat{\sigma}^{2}_{t-1}(\hat\bbx_{t})).
%
%
\end{align}
%
%Add subtract the term $\frac{1}{2} \sum^{T}_{t=1}\log(1+\sigma^{-2}{\sigma}^{2}_{T-1}(\bbx_{T}))$, we get 
%\begin{align}\label{third1}
%%
%%
%\mathbf{H}(\hat\bby_{T}) 
%=& \frac{1}{2}\sum^{T}_{t=1}\log(2\pi e\sigma^{2})+\frac{1}{2} \sum^{T}_{t=1}\log(1+\sigma^{-2}{\sigma}^{2}_{T-1}(\bbx_{T}))\nonumber
%\\
%&+\frac{1}{2} \sum^{T}_{t=1}\log\left(\frac{1+\sigma^{-2}\hat{\sigma}^{2}_{T-1}(\bbx_{T})}{1+\sigma^{-2}{\sigma}^{2}_{T-1}(\bbx_{T})}\right).
%%
%%
%\end{align}
From the update in \eqref{information}, it holds that
\begin{align}\label{fourth}
%
%
I(\hat\bby_{T};\hat\bbf_{T})=& 
\frac{1}{2} \sum_{t\in M_T(\epsilon)}\log(1+\sigma^{-2}\hat{\sigma}^{2}_{t-1}(\hat\bbx_{t})).
%\\
%&+\frac{1}{2} \sum^{T}_{t=1}\log\left(\frac{1+\sigma^{-2}\hat{\sigma}^{2}_{T-1}(\bbx_{T})}{1+\sigma^{-2}{\sigma}^{2}_{T-1}(\bbx_{T})}\right).
%%
%%
\end{align} 
%From the expression in \eqref{first} and \eqref{second}, we obtain the information gain expression presented in the statement of Lemma \ref{lemma3}. 
%At this step, no conclusion can be drawn about the effect of the compression sub-routine on the information gain which depends on the posterior covariance $\hat{\sigma}_{t}(x_{t})$.
\end{proof}
%\begin{lemma}
%	Pick $\delta \in (0,1)$ and let $\beta_{t}$ be defined as in Lemma 1 as $\beta_{t} = \log(|D|t^{2}\pi^{2}/6\delta)$, then with probability $1-\delta$, the following holds
%%%%%%%%%%%%%%%%%%%%%%%%%%%%%%%%%%%%%%%%%%%%%%%%%%%%%%%%%%%%%%%%%%%%%%%%%%%%%%%%%%%%%%%%%%%%%%%%%%%%%%%%%%%%%%%%%%%%%%%%%%%%%%%%%%%%%%%%%%%%%%%%%%%T H E O R E M%%%%%%%%%%%%%%%%%%%%%%%%%%%%%%%%%%%%
%%%%%%%%%%%%%%%%%%%%%%%%%%%%%%%%%%%%%%%%%%%%%%%%%%%%%%%%%%%%%%%%%%%%%%%%%%%%%%%%%%%%%%%%%%%%%%%%%%%%%%%%%%%%%%%%%%%%%%%%%%%%%%%%%%%%%%%%%%
\begin{lemma}
Pick $\delta\in(0,1)$ and let $\beta_t$ be defined as in Lemma \ref{lemma1}. Then , the following holds with probability $\geq 1-\delta$:
\begin{align}
\sum\limits_{t=1}^{T}r_t^2\leq \beta_T C
\end{align}
\end{lemma}
%
%
\begin{proof}
%
By Lemma \ref{lemma1} and \ref{lemma2}, we have 
%
\begin{align}\label{regret}
r_{t}^{2} \leq 4\beta_{t}\hat{\sigma}_{t-1}^{2}(\hat\bbx_{t})
\end{align}
%
 for all $t$ and holds with probability $1-\delta$. Since $\beta_{t}$ is non-decreasing, we obtain
%
\begin{align}
%
4\beta_{t}\hat{\sigma}_{t-1}^{2}(\hat\bbx_{t}) \leq 4\beta_{T}\sigma^2(\sigma^{-2}\hat{\sigma}_{t-1}^{2}(\hat\bbx_{t})).
%
\end{align}
%
%\begin{align}
%%
%\sum^{T}_{t=1} r_{t}^{2} \leq C_{1}\beta_{T}I(y_{T};f_{T}) \leq C_{1}\beta_{T}y_{T}
%%
%	\end{align}
%	%
%
In addition, note that, by definition, we restrict $\kappa(\bbx,\bbx') \leq 1$. Thus, $\hat{\sigma}^{2}_{t-1}(\hat\bbx_{t}) = \kappa(\hat\bbx_{t},\bbx_{t}) \leq 1$ for all $t$. Furthermore, 
using the fact that $\frac{s}{\log(1+s)}$ is monotonically increasing for positive $s$, we get
%
\begin{align}
%
\frac{\sigma^{-2}\hat{\sigma}^{2}_{t-1}(\hat\bbx_{t})}{\log(1+\sigma^{-2}\hat{\sigma}^{2}_{t-1}(\hat\bbx_{t}))} \leq \frac{\sigma^{-2}}{\log(1+\sigma^{-2})}.
%
\end{align} 
This implies that
\begin{align}
%
{\sigma^{-2}\hat{\sigma}^{2}_{t-1}(\hat\bbx_{t})} \leq \frac{\sigma^{-2}}{\log(1+\sigma^{-2})}{\log(1+\sigma^{-2}\hat{\sigma}^{2}_{t-1}(\hat\bbx_{t}))}.
%
\end{align} 
%
Multiplying both sides by $4\beta_{T}\sigma^{2}$, we obtain
%
\begin{align}\label{upper_bound}
%
4\beta_{T}\hat{\sigma}^{2}_{t-1}(\hat\bbx_{t})%
\leq 4\beta_{T}C_{2} \log(1+\sigma^{-2}\hat{\sigma}^{2}_{t-1}(\hat\bbx_{t}))
%
\end{align}
%
where $C_{2} = \frac{\sigma^{-2}}{\log(1+\sigma^{-2})}$. Next, substitute the upper bound in \eqref{upper_bound} on the right hand side of \eqref{regret}, we get 
%square the both sides and sum over all $t$, we get
%
%where $C_{1} = 8/\log(1+\sigma^{-2}) \geq 8\sigma^{2}$ and $\beta_{T}$ is $\beta_{t}$ at $t=T$. Using the lemmas above, we can obtain
\begin{align}
%
%\begin{split}
%
\sum^{T}_{t=1}r_{t}^{2} &\leq 4\beta_{T}{\sigma}^{2}C_{2}\sum^{T}_{t=1}\log(1+\sigma^{-2}\hat{\sigma}^{2}_{t-1}(\hat\bbx_{t}))
\end{align}
From the result in Lemma \ref{lemma3} and defining $C_1=8\sigma^2C_2$, we can write
\begin{align}
\sum^{T}_{t=1}r_{t}^{2}&\leq \beta_{T}C_{1}\left[I(\hat\bby_{T};\hat\bbf_{T})+\epsilon(T-M_T(\epsilon))\right]\nonumber\\
&\leq \beta_{T}C_{1}\left[I(\hat\bby_{T};\hat\bbf_{T})+\epsilon T\right].
%\\
%&\leq \beta_{T}C_{1}I(\bby_{T};\bbf_{T}).
%
%\end{split}
%
\end{align}

\subsection{General Decision Set} Now, we extend the results of Theorem 1 to the general settings where $\mathcal{A}\subset \mathcal{R}^d$ is a compact set. The result in Lemma \ref{lemma1} does not hold for infinite action space $\mathcal{A}$. Hence, we first need to state the equivalent result to Lemma \ref{lemma1} for the general case as follows. 

\begin{lemma}\label{lemma4}
Let $\delta\in(0,1)$ and set $\beta_t=2\log(\pi_t/\delta)$ such that $\sum\limits_{t\geq}\frac{1}{\pi_t}=1,  \pi_t>0$. Then, it holds that
\begin{align}
|f(\hat \bbx_t)-\hat\mu_{t-1}|\leq \beta_t^{1/2}\hat\sigma_{t-1}(\hat\bbx_t), \ \ \forall t\geq 1
\end{align}
holds with probability $\geq 1-\delta$.
\end{lemma}
\begin{proof}
For a given $t$ and $\bbx\in\mathcal{A}$, the dictionary $\bbD_{t-1}$ elements are deterministic conditioned on the observations $\hat \bby_{t-1}$, which implies that $f(\bbx)\sim\mathcal{N}(\hat\mu_{t-1(\bbx)},\hat{\sigma}^2_{t-1}(\bbx))$. Following the similar steps to the proof of Lemma \ref{lemma1}, it holds that 
\begin{align}
%
P\Big\{|f(\hat\bbx_t)-\hat{\mu}_{t-1}(\hat\bbx_t)|&>\beta_{t}^{1/2}\hat{\sigma}_{t-1}(\hat\bbx_t)\Big\}\leq e^{-\beta_{t}/2}.
%
\end{align}
Since we have $\beta_t=2\log(\pi_t/\delta)$ and utilizing the union bound for $t\in\mathbb{N}$, we get the statement of Lemma \ref{lemma4}.
\end{proof}
%
%Next, from the equality in \eqref{fourth}, we get 
%\begin{align}
%%
%%\begin{split}
%%
%\sum^{T}_{t=1}r_{t}^{2} \leq& \beta_{T}C_{1}\left(I(\bby_{T};\bbf_{T})+\bbH(\hat{\bby}_t)-\bbH({\bby}_t)\right)\nonumber
%\\
%\leq&\beta_{T}C_{1}I(\bby_{T};\bbf_{T})\nonumber 
%\\ &+\beta_{T}C_{1}\left(\frac{1}{2} \sum^{T}_{t=1}\log\left(\frac{1+\sigma^{-2}\hat{\sigma}^{2}_{t-1}(\bbx_{t})}{1+\sigma^{-2}{\sigma}^{2}_{t-1}(\bbx_{t})}\right)\right).
%%
%%\end{split}
%%
%\end{align}
%\red{The only remaining challenge is to link the last term to the Hellinger or any other kind of metric of distance between the Gaussian distributions. This is important to incorporate the factor of compression budget $\epsilon$ in the final expression.  I will look at that tomorrow. }

%the POG algorithm, we know the probability distributions corresponding to the real variance $\sigma_{t-1}(x_{t}$ and the compressed variance $\hat{\sigma}_{t-1}(x_{t}$ are $\epsilon_{t}$ apart, where $\epsilon$ is the compression budget. Therefore, we can represent the final regret bounds in terms of the real variance and the compression budget. \red{This  is not correct, because the metric in which they are close is not properly incorporated.} This is represented as

%\begin{equation}
%%
%\begin{split}
%%
%\sum^{T}_{t=1}r_{t}^{2} \leq 4\beta_{T}{\sigma}^{2}C_{2}\sum^{T}_{t=1}\log{\big(1+\sigma^{-2}({\sigma}^{2}_{t-1}(x_{t})+k\epsilon^{2}_{t})\big)}
%%
%\end{split}
%%
%\end{equation}
%%
%where $k$ is a constant. 
%
%Next, consider the cumulative regret squared
%%
%\begin{align}
%%
%R^{2}_{T} =& \left(\sum^{T}_{t=1}r_{t}\right)^{2} \leq T\sum^{T}_{t=1}r^{2}_{t}
%\\
% \implies R_{T} \leq& \sqrt{T\sum_{t=1}^{T}r^{2}_{t}}
%%
%\end{align}
%
%This concludes the proof of the theorem.
\end{proof} 

\begin{theorem}\label{model_order}
We need to prove that $M_T(\epsilon)\rightarrow M_{\infty}$ as $T\rightarrow \infty$ where $M_{\infty}$ is some constant $M_{\infty}<\infty$. Further, we can characterize the constant as 
\begin{align}\label{upper_bound2}
   M_{\infty}\leq Y(CH)^p\left(\frac{\eta}{\epsilon}\right)^p.
\end{align} 
\end{theorem}
 
\begin{proof}
%  Before proving Lemma \ref{theorem_model_order}, we present a lemma which allows us to relate the stopping criterion of our sparsification procedure to a Hilbert subspace distance.
% %\red{discussion of lemma}
% %%%%%%%%%%%%%%%%%%%%%%%%%%%%%%%%%%%%%%%%%%%%%%%%%%%%%%%%%%%%%%%
% %%% L  E  M  M  A  %%%%%%%%%%%%%%%%%
% %%%%%%%%%%%%%%%%%%%%%%%%%%%%%%%%%%%%%%%%%%%%%%%%%%%%%%%%%%%%%%%
% %
% \begin{lemma}\label{lemma_subspace_dist}
% Define the distance of an arbitrary feature vector $\bbx$ evaluated by the feature transformation $\phi(\bbx) = \kappa(\bbx, \cdot)$ to $\ccalH_{\bbD}=\text{span}\{\kappa(\bbd_t, \cdot) \}_{t=1}^M$, the subspace of the Hilbert space spanned by a dictionary $\bbD$ of size $M$,  as
% %
% \begin{align}\label{eq:hilbert_subspace_dist}
% %
% \text{dist}( \kappa(\bbx, \cdot) , \ccalH_{\bbD}) 
% = \min_{f\in\ccalH_{\bbD}} \| \kappa(\bbx, \cdot) - \bbv^T \bbkappa_{\bbD}(\cdot) \|_{\ccalH} \; .
% %
% \end{align}
% %
% This set distance simplifies to following least-squares projection when $\bbD \in \reals^{p\times M}$ is fixed
% %
% \begin{align}\label{eq:hilbert_subspace_dist_ls}
% \text{dist}( \kappa(\bbx, \cdot) , \ccalH_{\bbD}) 
% = \Big\|  \kappa(\bbx,\cdot) 
%   - [\bbK_{\bbD, \bbD}^{-1} \bbkappa_{\bbD}(\bbx)]^T
%    \bbkappa_{\bbD}(\cdot) \Big\|_{\ccalH} \; .
% \end{align}
% %
% \end{lemma}
% 
% 
% 
% %%%%%%%%%%%%%%%%%%%%%%%%%%%%%%%%%%%%%%%%%
% %%%%%%%%%%%%%%%%%%%%%%%%%%%%%%%%%%%%%%%%%
% %%%%%%%%    P   R   O   O   F    %%%%%%%%%%%%%%%%%%%%%%% 
% %%%%%%%%%%%%%%%%%%%%%%%%%%%%%%%%%%%%%%%%%
% %%%%%%%%%%%%%%%%%%%%%%%%%%%%%%%%%%%%%%%%%
% %\begin{proof} See Appendix 
% 
% %We now present our main result, which says that the model order of $f_t$ remains bounded for all $t$, and depends on the conditioning of the problem setting as well as the feature space.
% 
% %\subsection{Proof of Lemma \ref{lemma_subspace_dist}}\label{apx_lemma_subspace_dist}
% %%%%%%%%%%%%%%%%%%%%%%%%%%%%%%%%%%%%%%%%%
% %%%%%%%%%%%%%%%%%%%%%%%%%%%%%%%%%%%%%%%%%
% %%%%%%%%    P   R   O   O   F    %%%%%%%%%%%%%%%%%%%%%%% 
% %%%%%%%%%%%%%%%%%%%%%%%%%%%%%%%%%%%%%%%%%
% %%%%%%%%%%%%%%%%%%%%%%%%%%%%%%%%%%%%%%%%%
% \begin{proof}
% The distance to the subspace $\ccalH_{\bbD}$ is defined as
% %
% \begin{align}\label{eq:subspace_dist}
% %
% \text{dist}( \kappa(\bbx, \cdot) , \ccalH_{\bbD_t}) 
% =& \min_{f\in\ccalH_{\bbD}} \| \kappa(\bbx, \cdot) - \bbv^T \bbkappa_{\bbD}(\cdot) \|_{\ccalH}\nonumber\\ 
% =& \min_{\bbv\in \reals^{M}} \| \kappa(\bbx, \cdot) - \bbv^T \bbkappa_{\bbD}(\cdot) \|_{\ccalH} \; ,
% %
% \end{align}
% %
% where the first equality comes from the fact that the dictionary $\bbD$ is fixed, so $\bbv\in \reals^M$ is the only free parameter. Now plug in the minimizing weight vector $\tbv^\star=\bbK_{\bbD_t, \bbD_t}^{-1}\bbkappa_{\bbD_t}(\bbx_t)$ into \eqref{eq:subspace_dist} which is obtained in an analogous manner to the logic which yields \eqref{eq:hatparam_update}. Doing so simplifies \eqref{eq:subspace_dist} to the following
% %
% \begin{align}\label{eq:subspace_dist2}
% %
% \text{dist}(\kappa(\bbx_t, \cdot) , \ccalH_{\bbD_t}) \!=\!  \Big\|  \kappa(\bbx_t,\cdot) 
%   - [\bbK_{\bbD_t, \bbD_t}^{-1} \bbkappa_{\bbD_t}(\bbx_t)]^T
%    \bbkappa_{\bbD_t}(\cdot) \Big\|_{\ccalH} \; .
% %
% \end{align}
% %
% \end{proof}
% %%%%%%%%%%%%%%%%%%%%%%%%%%%%%%%%%%%%%%
% %%%%%%%%%%%%%%%%%%%%%%%%%%%%%%%%%%%%%
% %%%%%%%%%   S  E   C   T   I    O    N    %%%%%%%%%%%%%%%
% %%%%%%%%%%%%%%%%%%%%%%%%%%%%%%%%%%%%%
% %%%%%%%%%%%%%%%%%%%%%%%%%%%%%%%%%%%%%
% \subsection{Proof of Lemma \ref{theorem_model_order}}\label{apx_theorem_model_order}
 %%%%%%%%%%%%%%%%%%%%%%%%%%%%%%%%%%%%%%%%%
 %%%%%%%%%%%%%%%%%%%%%%%%%%%%%%%%%%%%%%%%%
 %%%%%%%%    P   R   O   O   F    %%%%%%%%%%%%%%%%%%%%%%% 
 %%%%%%%%%%%%%%%%%%%%%%%%%%%%%%%%%%%%%%%%%
 %%%%%%%%%%%%%%%%%%%%%%%%%%%%%%%%%%%%%%%%%
 %\begin{proof}
 %
Consider the model order of the dictionary $\bbD_{t-1}$ at $t-1$ and $\bbD_{t}$ generated by Algorithm \ref{alg:compressed} denoted by $M_{t-1}$ and $M_{t}$, respectively, at two arbitrary subsequent times $t-1$ and $t$. The number of elements in $\bbD_{t-1}$ are $M_{t-1}=(t-1)$. After performing the algorithm update at $t$, we add a new data points to the dictionary and increase the model order by one, hence $M_{t}=M_{t-1}+1$. Hence, there are only two possibilities, wither we increase $M_{t-1}$ by $1$ at $t$ or not which means $M_{t}=M_{t-1}$.
 %
% Specifically, rather than allowing the dimension of the Hilbert subspace to which $f$ belongs to grow by $1$ at each time as in \eqref{eq:param_update}, we propose to project them onto time-varying subspaces generated by dictionaries $\bbD=\bbD_{t+1}$ extracted from the data points observed thus far.
 
%   Begin by assuming function ${f}_{t+1}$ is parameterized by dictionary $\bbD_{t+1}$ and weight vector $\bbw_{t+1}$. Moreover, we denote columns of $\bbD_{t+1}$ as $\bbd_t$ for $t=1,\dots,{M}_{t+1}$.
 %
 % Assume a constant algorithm step-size $\eta$ has been chosen such that $\eta<1/\lambda$ and the approximation budget $\eps$ satisfies $\eps=K \eta^{3/2}$ for some positive scalar $K>0$.
 %
 Suppose the model order $M_{t}$ is equal to that of $M_{t-1}$, i.e. $M_{t} = M_{t-1}$. This relation holds when $\mathbf{H}(y_{t}|\hat\bby_{t-1}) > \eps$, \emph{is not} satisfied for the new information with the newest data point $y_t$.
 %
 Thus, the negation holds for this case, stated as
 %
 \begin{align}\label{eq:komp_to_terminate}
 \mathbf{H}(y_{t}|\hat\bby_{t-1})  \leq \eps \; .
 \end{align}
 %
  Consequently, if $\mathbf{H}(y_{t}|\hat\bby_{t-1})$, then \eqref{eq:komp_to_terminate} holds and the model order does not grow. Thus it suffices to consider $\mathbf{H}(y_{t}|\hat\bby_{t-1})$.
 
   
 
 Now, let's take the contrapositive of the preceding expressions to observe that growth in the model order ($M_{t} = M_{t-1} + 1$) implies that the condition
 %
 \begin{align}
  \label{eq:min_gamma2}
  \hat{\sigma}^{2}_{t-1}(\hat\bbx_{t}) > \frac{\exp(2\epsilon)}{2\pi e}-\sigma^{2}
  \end{align} %\vspace{-5cm}
 %
 holds. The above expression implies that 
 \begin{align}
 1-{\boldsymbol{\kappa}}_{{{\bbD}}_{t-1}}(\hat\bbx_{t})^T(\bbK_{t-1}+\sigma^{2}\bbI)^{-1}{\boldsymbol{\kappa}}_{{{\bbD}}_{t-1}}(\hat\bbx_{t})> \frac{\exp(2\epsilon)}{2\pi e}-\sigma^{2}
 \end{align}
 
 
  Therefore, each time a new point is added to the model, the corresponding kernel function is guaranteed to be at least a distance of {$\frac{\epsilon}{\eta|\check L_t'({f}_t(\bbx_t)) |}$} from every other kernel function in the current model. 
 
 
 By the $C$-Lipschitz continuity of the instantaneous loss (Assumption \ref{as:2}): specifically {$1/|\nabla_f \check{L}_t (f_{t}(\bbS_t))| \geq 1/HC$}, we can lower-bound the threshold condition in \eqref{eq:min_gamma2} as 
 %
 \begin{align}\label{eq:min_gamma3}
  %
   \frac{\epsilon}{\eta|\check\ell_t'({f}_t(\bbx_t)) |}\geq \frac{\epsilon}{\eta CH}
   %
  \end{align}
 %
 We have
  \begin{align}
  \label{eq:min_gamma321}
  \text{dist}(\kappa(\bbx_t,\cdot),\ccalH_{\bbD_t}) > \frac{\epsilon}{\eta CH}
  \end{align}
  %
 Therefore, For a fixed compression budget $\epsilon$ and step size $\eta$, the KOMP stopping criterion is violated for the newest point whenever distinct dictionary points $\bbd_k$ and $\bbd_j$  for $j,k\in\{1,\dots,M_t\}$, satisfy the condition $\|\phi(\bbd_j) - \phi(\bbd_k) \|_\mathcal{H} > \frac{\epsilon}{\eta CH}$. Next, we follow the similar argument as provided in the proof of Theorem 3.1 in \citep{1315946}.   Since $\ccalX$ is compact and $\kappa$ is continuous, the range $\phi(\ccalX) $ (where $\phi(\bbx)=\kappa(\bbx,\cdot)$ for $\bbx \in \ccalX$) of the kernel transformation of feature space $\ccalX$ is compact.   Therefore, the number minimum of balls (covering number) of radius $\delta$ (here, $\delta = \frac{\epsilon}{\eta CH}$) needed to cover the set $\phi(\ccalX)$ is finite (see, e.g., \citep{anthony2009neural}) for a fixed compression budget $\epsilon$ and step-size $\eta$.
 
 % Further for the non-stationary settings, we select the compression budget $\epsilon$ to be inversely proportional to $T$ in order to make regret sublinear, which implies that the radius of $\delta$ balls is going to zero with $T$. Hence, the covering number approaches infinite. Under this condition, it becomes important to study the rate at which the size of the dictionary increases with respect to decrease in the compression budget. 
  To arrive at the characterization detailed in Theorem \ref{model_order}, we note that \citep[Proposition 2.2]{1315946} states that for a Lipschitz continuous Mercer kernel $\kappa$ on compact set $\mathcal{X}\subseteq\mathbb{R}^p$, there exists a constant $Y$ such that for any training set $\{\bbx_t\}_{t=1}^\infty$ and any $\nu>0$, and it holds for  the number of elements in dictionary that  %\blue{Really interesting... this result is definitely missing from the literature: exactly relating model complexity to compression budget/step-size selection is really interesting. That we have to better accentuate in the {\bf Contribution} discussion in Sec. \ref{sec:Problem}. }
  %
  \begin{align}\label{model_order_1}
  %
  M\leq Y\left(\frac{1}{\nu}\right)^p.
  %
  \end{align}
  %
 where $Y$ is a constant depends upon $\mathcal{X}$ and the kernel function. By \eqref{eq:min_gamma321}, we have that $\nu=\frac{\epsilon}{\eta CH}$, which we may substitute into \eqref{model_order_1} to obtain
  %
  \begin{align}\label{model_order_2}
  %
   M\leq Y(CH)^p\left(\frac{\eta}{\epsilon}\right)^p.
   %
   \end{align}
   %
   as stated in \eqref{model_order_0}. The lower bound $H$ in \eqref{model_order_0} comes from the fact that to represent the instantaneous gradient of the windowed loss of length $H$, a minimum of $H$ points are required.  \hfill %  Then, the model order of the learned function will depend on the ratio of the step-size to the compression budget, problem constants such as Lipschitz continuity modulus and the parsimony constant.
  % From the above expression, we will get different upper bounds for the different decrement rate of the compression budget  which we will choose in accordance with to minimize the regret. The result in \eqref{model_order_1} holds directly for POLK and related the tradeoff between stepsize and compression budget for POLK. This result was missing from POLK. 
 %
 %\end{proof}
\end{proof}
%Next, consider the general case where $D \in \mathbb{R}^{d}$ is any compact and convex set. Note that since we deal with a continuous set, the lemmas considered before will not be directly applicable since they are a function of size of $D$. The regret bounds for this case requires additional assumptions on the kernel function.

%\begin{lemma}
%	Choose $\delta \in (0,1)$ and let $\beta_{t} = 2\log(|2\pi_{t}/\delta)$, for some $\pi_{t}$ such that $\sum_{t\geq 1} \pi_{t}^{-1} = 1, \pi_{t} >0$. Then
%	\begin{align}
%	|f(\bbx)-{t-1}(\bbx)| \leq \beta_{t}^{1/2}\sigma_{t-1}(\bbx)\hspace{0.1in} \forall \bbx \in D, \forall t \geq 1
%	\end{align}
%	holds with probability $\geq 1-\delta$.
%\end{lemma}
%The proof is similar to the Lemma 1 except we dont have the function of size of $D$ although it is possible to divide $D$ into finite sets. 
%\begin{lemma}
%	Pick $\delta \in (0,1)$ and set $\beta_{t} = 2\log(2\pi_{t}/\delta)+4d\log{(dtbr\sqrt{\log(2da/\delta)}}$, where $\sum_{t\geq1}\pi^{-1}_{t} = 1, \pi_{t} >0$.Let $\tau_{t} = dt^{2}br^{2}\sqrt{\log(2da/\delta)}$. Let $[x^{\star}]_{t}$ denote the closest point in $D_{t}$ to $x^{\star}$. Then,
%	\begin{align}
%	|f(x^{\star})-{t-1}(|x^{\star}|_{t})\leq \beta^{1/2}_{t}\sigma_{t-1}(|x^{\star}|_{t})+\frac{1}{t^{2}}, \forall t \geq 1
%	\end{align}
%\end{lemma}

%%!TEX root = main.tex
%%%%%%%%%%%%%%%%%%%%%%%%%%%%%%%%%%%%%%%%%%%%%%%%%%%%%%%%%%%%%%%%%%%%%%%%%%%%%%%%%%%%%%%%%%% S  E  C  T  I  O  N %%%%%%%%%%%%%%%%%%%%%%%%%%%%%%%%%%%%%%%%%%%%%%%%%%%%%%%%%%%%%%%%%%%%%%%%%%%%%%%%%%%%%%%%%%%%%%%%%%%%%%%%%%%%%%%%%%%%%%%%%%%%%%%%%%%%%%%%%%%%%%%%%%%%%%%%%%%%%%%%%%%%%%%%%%%%%%%%%%%%%%%%%%
%%
%
%%!TEX root = main.tex
%%%%%%%%%%%%%%%%%%%%%%%%%%%%%%%%%%%%%%%%%%%%%%%%%%%%%%%%%%%%%%%%%%%%%%%%%%%%%%%%%%%%%%%%%%% S  E  C  T  I  O  N %%%%%%%%%%%%%%%%%%%%%%%%%%%%%%%%%%%%%%%%%%%%%%%%%%%%%%%%%%%%%%%%%%%%%%%%%%%%%%%%%%%%%%%%%%%%%%%%%%%%%%%%%%%%%%%%%%%%%%%%%%%%%%%%%%%%%%%%%%%%%%%%%%%%%%%%%%%%%%%%%%%%%%%%%%%%%%%%%%%%%%%%%%
%%
%\section{Consistent Compressions of Gaussian Processes}
%
%\blue{
%\begin{enumerate}
%%
%%\item 
%%
%%\item talk about a few natural approaches for regular (frequentist) bandits (vanilla UCB, Gittens indices, knowledge gradient) and how Bayesian bandit algs are different. We focus on UCB due to its simplicity, and Bayesian variant due to its ability to conduct efficient exploration.$\rightarrow$ Need to be careful about word usage of efficient exploration, and reference some Van Roy papers on the topic. Efficient exploration means we don't need to do uniform sampling, but instead can do it according to posterior distribution.
% %
%%\item   Then present basic GP-UCB algorithm and give as lemmas the existing regret bounds for vanilla GP UCB. 
%%
%%\item then discuss how the GP-UCB algorithm suffers from the usual curse of dimensionality in nonparametric statistics (we can citep POLK, POG, importance samgling, or the SPM paper)
%
%\item To avoid curse of dimensionality, we propose information-gain based rule to deciding when a point enters into posterior. This allows us to trade off regret and complexity. That's the focus of Section IV.
%\end{enumerate}}
%%
% The GP-UCB algorithm is expressed as
%
%
%\begin{algorithm}[t]
%\label{alg:compressed}
%%
%	\caption{Compressed GP-UCB Algorithm (CUB)}\label{alg:cub}
%	%
%	\begin{algorithmic}
%	%
%		\FOR{t = 1,2...}
%		%
%		\STATE Find $\hat\bbx_{t}$ by solving an optimization problem: $$\hat\bbx_{t} = \arg\max_{\bbx\in\mathcal{A}}
%		 \hat\mu_{t-1}(\bbx)+\sqrt{\beta_t}\hat\sigma_{t-1}(\bbx)$$\\
%		 
%		% We have a distribution $\hat{\mathcal{G}}_{t-1}=\mathcal{N}(\hat{\mu}_{t-1}(\bbx),\hat\sigma_{t-1}^{2}(\bbx))$
%		%
%		\STATE Sample: $\hat y_{t} = f(\hat\bbx_{t})+\epsilon_{t}$
%		%
%		 \STATE{\bf If} info. gain exceeds $\epsilon$ threshold $\mathbf{H}(y_{t}|\hat\bby_{t-1})=\frac{1}{2}\log\big(2\pi e(\sigma^{2}+\hat{\sigma}^{2}_{t-1}(\hat\bbx_{t}))\big)>\epsilon$
%		\INDSTATED Augment dictionary ${{\bbD}}_{t} = \{{{\bbD}}_{t-1};(\hat\bbx_{t},\hat y_{t})\}$
%			\INDSTATED Update posterior mean $\tilde{\mu}_{t}(\bbx)$ and variance $\tilde{\sigma}_{t}(\bbx)$ 
%		%
%		\begin{align*}
%		\hat{\mu}_{t}(\bbx)=&{\boldsymbol{k}}_{{{\bbD}}_{t}}(\bbx)^{T}(\bbK_{T}+\sigma^{2}\bbI)^{-1}\bby_{{{\bbD}}_{t}}&
%		%
%		\\		\hat\sigma_{t}^{2}(\bbx)=&\kappa(\bbx,\bbx^{\prime})-{\boldsymbol{k}}_{{{\bbD}}_{t}}(\bbx)^T(\bbK_{T}+\sigma^{2}\bbI)^{-1}{\boldsymbol{k}}_{{{\bbD}}_{t}}(\bbx^{\prime})
%		%\\
%		%\hat\sigma_{t}^{2}(\bbx)=&\kappa_{t}(\bbx,\bbx) 
%				\end{align*}
%				\vspace{-8mm}
%		\STATE{\bf Else} 
%		\INDSTATED Dictionary $\bbD_t= \bbD_{t-1}$ and GP remain unchanged
%		$$(\hat\mu_t(\bbx),\hat{\sigma}_{t}(\bbx),{\bbD}_{t})=(\hat\mu_{t-1}(\bbx),\hat{\sigma}_{t-1}(\bbx),{\bbD}_{t-1})$$
%		\ENDFOR
%		%
%	\end{algorithmic}
%	%
%\end{algorithm}
%
%
%
%\section{Proposed Algorithm}
% The GP-UCB algorithm is expressed as
%
%
%%\begin{algorithm}
%%%
%%	\caption{Compressed GP-UCB Algorithm (CGP-UCB)}\label{alg:euclid}
%%	%
%%	\begin{algorithmic}
%%	%
%%		\FOR{t = 1,2...}
%%		%
%%		\STATE Find $\hat\bbx_{t}$ by solving an optimization problem: $$\hat\bbx_{t} = \arg\max_{\bbx\in\mathcal{A}}
%%		 \hat\mu_{t-1}(\bbx)+\sqrt{\beta_t}\hat\sigma_{t-1}(\bbx)$$\\
%%		 
%%		 We have a distribution $\hat{\mathcal{G}}_{t-1}=\mathcal{N}(\hat{\mu}_{t-1}(\bbx),\hat\sigma_{t-1}^{2}(\bbx))$
%%		%
%%		\STATE Sample: $\hat y_{t} = f(\hat\bbx_{t})+\epsilon_{t}$\\
%%		%
%%		\STATE Augment data ${\tilde{\bbD}}_{t} = \{{{\bbD}}_{t-1};(\hat\bbx_{t},\hat y_{t})\}$\\
%%		%
%%		\STATE Update posterior mean $\tilde{\mu}_{t}(\bbx)$ and variance $\tilde{\sigma}_{t}(\bbx)$ 
%%		
%%		\begin{align}
%%		\tilde{\mu}_{t}(\bbx)=&{\boldsymbol{\kappa}}_{{\tilde{\bbD}}_{t}}(\bbx)^{T}(\bbK_{T}+\sigma^{2}\bbI)^{-1}\bby_{{\tilde{\bbD}}_{t}}&
%%		\\ k_{t}(\bbx,\bbx^{\prime})=&\kappa(\bbx,\bbx^{\prime})-{\boldsymbol{\kappa}}_{{\tilde{\bbD}}_{t}}(\bbx)^T(\bbK_{T}+\sigma^{2}\bbI)^{-1}{\boldsymbol{\kappa}}_{{\tilde{\bbD}}_{t}}(\bbx^{\prime})\nonumber
%%		\\
%%		\tilde\sigma_{t}^{2}(\bbx)=&\kappa_{t}(\bbx,\bbx) 
%%				\end{align}
%%				
%%				We get a new  distribution $\tilde{\mathcal{G}}_{t}=\mathcal{N}(\tilde{\mu}_{t}(\bbx),\tilde\sigma_{t}^{2}(\bbx))$
%%		\STATE Compress mean and covariance to get mean $
%%		{\tilde\mu}_t(\bbx)$ and covariance ${\tilde\sigma}_{t}(\bbx)$ and dictionary $\tilde{\bbD}_{t}$ 
%%		%
%%	 $$(\hat\mu_t(\bbx),\hat{\sigma}_{t}(\bbx),{\bbD}_{t})=\text{Compress}(\tilde\mu_t(\bbx),\tilde{\sigma}_{t}(\bbx),\tilde{\bbD}_{t})$$
%%		%
%%		such that $d_H(\hat{\mathcal{G}}_{t},\tilde{\mathcal{G}}_{t})\leq \epsilon.$
%%		\ENDFOR
%%		%
%%	\end{algorithmic}
%%	%
%%\end{algorithm}
%
%Consider the case where the domain $\mathcal{A}$ is of finite size $|\mathcal{A}|$. 
%
%\section{Regret Bounds}
%
%To prove the regret bounds for the proposed algorithm, we consider the different settings of finite decision set $\mathcal{A}$ with $f\sim \text{GP}(0,\kappa(\bbx,\bbx'))$, general compact set $\mathcal{A}$ with $f\sim \text{GP}(0,\kappa(\bbx,\bbx'))$, and  when $f$ belongs to RKHS with bounded norm (\red{last one, still need to decide}).
%\subsection{Finite Decision Set}
%
%%%%%%%%%%%%%%%%%%%%%%%%%%%%%%%%%%%%%%%%%%%%%%%%%%%%%%%%%%%%%%%%%%%%%%%%%%%%%%%%%%%%%%%%%%%%%%%%%%%%%%%%%%%%%%%%%%%%%%%%%%%%%%%%%%%%%%%%%%%%%%%%%%%%T H E O R E M%%%%%%%%%%%%%%%%%%%%%%%%%%%%%%%%%%%%
%%%%%%%%%%%%%%%%%%%%%%%%%%%%%%%%%%%%%%%%%%%%%%%%%%%%%%%%%%%%%%%%%%%%%%%%%%%%%%%%%%%%%%%%%%%%%%%%%%%%%%%%%%%%%%%%%%%%%%%%%%%%%%%%%%%%%%%%%%%
%%\begin{theorem}\label{thm:1}
%%%
%%	Let $\delta \in (0,1)$ and $\beta_{t} = 2\log(|\mathcal{A}|t^{2}\pi^{2}/6\delta)$. Running the GP-UCB algorithm shown in Algorithm 2, we obtain the following regret bound
%%	%
%%	\begin{align}\label{eq:regretbound_discrete_domain}
%%	%
%%	\text{Pr}\{R_{T} \leq \sqrt{T\sum_{t=1}^{T}\log{\big(1+\sigma^{-2}({\sigma}^{2}_{t-1}(x_{t})+k\epsilon^{2}_{t})\big)}} \hspace{0.1in} \forall T \geq 1\} \geq 1-\delta
%%	%
%%	\end{align}
%%	%
%%\end{theorem}
%%
%%where $C_{1} = \frac{8}{\log(1+\sigma^{-2})}$, $k$ is a constant and $\epsilon_{t}$ is the compression budget. Theorem~\ref{thm:1} is proved using the following sequence of lemmas. The proof is similar in spirit to that in~\citep'{srinivas2012information}. It is first shown that the absolute difference between the true function and the estimated mean obtained using the POG algorithm is upper bounded by the estimated variance function. This result is then used to bound the instantaneous regret in Lemma~\ref{lemma2}. We finally use this result to obtain the bounds on the cumulative regret.
%%
%%\blue{Here we need a short outline of the logic of the proof which will help the reader understand what's going on and how the lemmas relate to each other. Also note that I've observe that I've put commented out headers in front of important things, and put proof environments around the proofs, to make them more formal and discernible.}
%%%%%%%%%%%%%%%%%%%%%%%%%%%%%%%%%%%%%%%%%%%%%%%%%%%%%%%%%%%%%%%%%%%%%%%%%%%%%%%%%%%%%%%%%%%%%%%%%%%%%%%%%%%%%%%%%%%%%%%%%%%%%%%%%%%%%%%%%%%%%%%%%%%%L E M M A%%%%%%%%%%%%%%%%%%%%%%%%%%%%%%%%%%%%
%%%%%%%%%%%%%%%%%%%%%%%%%%%%%%%%%%%%%%%%%%%%%%%%%%%%%%%%%%%%%%%%%%%%%%%%%%%%%%%%%%%%%%%%%%%%%%%%%%%%%%%%%%%%%%%%%%%%%%%%%%%%%%%%%%%%%%%%%%%
%\begin{lemma}\label{lemma1}
%%
%	Choose $\delta \in (0,1)$ and let $\beta_{t} = 2\log(|\mathcal{A}|\pi_{t}/\delta)$, for some $\pi_{t}$ such that $\sum_{t\geq 1} \pi_{t}^{-1} = 1, \pi_{t} >0$. Then
%	%
%	\begin{align}\label{eq:lemma1}
%	%
%	|f(\bbx)-\hat{\mu}_{t-1}(\bbx)| \leq {\beta}_{t}^{1/2}\hat{\sigma}_{t-1}(\bbx)\hspace{0.1in} \forall \bbx \in \mathcal{A}, \forall t \geq 1
%	%
%	\end{align}
%	%
%	holds with probability $\geq 1-\delta$.
%	%
%	\end{lemma}
%	%
%	%%%%%%%%%%%%%%%%%%%%%%%%%%%%%%%%%%%%%%%%%%%%%%%%%%%%%%%%%%%%%%%%%%%%%%%%%%%%%%%%%%%%%%%%%%%%%%%%%%%%%%%%%%%%%%%%%%%%%%%%%%%%%%%%%%%%%%%%%%%%%%%%%%% P  R  O  O  F%%%%%%%%%%%%%%%%%%%%%%%%%%%%%%%%%%%%%%%%%%%%%%%%
%%%%%%%%%%%%%%%%%%%%%%%%%%%%%%%%%%%%%%%%%%%%%%%%%%%%%%%%%%%%%%%%%%%%%%%%%%%%%%%%%%%%%%%%%%%%%%%%%%%%%%%%%%%%%%%%%%%%%%%%%%%%%%%%%%%%%%%%%%%
%	\begin{proof}
%At each $t$, we have dictionary $\bbD_{t-1}$ which contains the data points for the function $f(\bbx)$. For a given $\bbD_{t-1}$, we  have $f(\bbx) \sim {N}(\hat{\mu}_{t-1},\hat{\sigma}_{t-1})$. Note that in the normal GP-UCB algorithm, since we are using compression at each time instant, we end up taking actions $\hat\bbx_{i=1:t}$ and observations $\hat y_{i=1:t}$ which are different from $\{\bbx_s\}_{s=1}^t$ and $\{y_s\}_{s=1}^t$ of the GP-UCB algorithm.  Hence, $(\hat{\mu}_{t-1},\hat{\sigma}_{t-1})$ defines a Gaussian distribution $\hat{\mathcal{G}}_{t-1}$ which is parametrized by the collection of data points $(\hat\bbx,\hat y)\in\bbD_{t-1}$. At $t$, we  take an action $(\hat \bbx_t)$ and observe $\hat y_t$. Then, we perform the update to obtain $(
%\tilde{\mu}_{t-1},\tilde{\sigma}_{t-1})$ which defines the distribution $\tilde{\mathcal{G}}_t$. Next, we drop the new data point to store in the dictionary if the new information $\mathbf{H}(y_{t}|\hat\bby_{t-1})\leq\epsilon$ where $\epsilon$ is the compression budget. Hence, there is a fundamental difference between both the algorithms and we seek to analyze the performance of the proposed algorithm in terms the regret defined against the optimal $f(\bbx^\star)$. For a random variable $r \sim N(0,1)$, the cumulative density function can be used to express
%%
%\begin{align}\label{eq:gaussian_tail_integration}
%%
%P(r>c) &= \frac{1}{\sqrt{2\pi}}\int_{c}^{\infty}e^{-\frac{r^2}{2}}dr\\
%%
% &= e^{\frac{-c^2}{2}}\frac{1}{\sqrt{2\pi}}\int_{c}^{\infty}e^{((\frac{-r^2}{2}+rc-\frac{c^2}{2})+(-rc-c^2))}dr \nonumber \\
%%
%&=e^{-\frac{c^2}{2}}\frac{1}{\sqrt{2\pi}}\int_{c}^{\infty}e^{-\frac{(r-c)^2}{2}}e^{-c(r-c)}dr. \nonumber
%%
%\end{align}
%%
%For $c > 0$ and $r\geq c$, we have that $e^{-c(r-c)}\leq 1$. Furthermore, the integral term scaled by $\frac{1}{\sqrt{2\pi}}$ resembles the Gaussian density integrated from $c$ to $\infty$ for a random variable $r$ with mean $c$ and unit standard deviation, integrated to $1/2$. Therefore, we get
%%
%\begin{align}\label{eq:gaussian_tail_approximation}
%%
%P(r>c) \leq e^{-c^{2}/2} P(r>0)=\frac{1}{2}e^{-c^{2}/2}.
%%
%\end{align}
%%
%Using the expression $r = (f(\bbx)-\hat{\mu}_{t-1}(\bbx))/\hat{\sigma}_{t-1}(\bbx)$  and $c = \beta_{t}^{1/2}$ for some sequence of nonnegative scalars $\{\beta_t\}_{t\geq 0}$ {substituted into the left-hand side of \eqref{eq:gaussian_tail_integration} using the left-hand side of \eqref{eq:gaussian_tail_approximation} }, we obtain
%%
%\begin{align}
%%
%P\Big\{|f(\bbx)-\hat{\mu}_{t-1}(\bbx)|&>\beta_{t}^{1/2}\hat{\sigma}_{t-1}(\bbx)\Big\}\leq e^{-\beta_{t}/2}.
%%
%\end{align}
%%
%Now apply Boole's inequality to the preceding expression to write
%%
%\begin{align}
%%
%P\Big\{{{\bigcup}}_{\bbx \in \mathcal{A}}& |f(\bbx)-\hat{\mu}_{t-1}(\bbx)|>\beta_{t}^{1/2}\hat{\sigma}_{t-1}(\bbx)\Big\}\nonumber
%\\
%&\leq \sum_{\bbx \in \mathcal{A}} P\Big\{|f(\bbx)-\hat{\mu}_{t-1}(\bbx)|>\beta_{t}^{1/2}\hat{\sigma}_{t-1}(\bbx)\Big\}\nonumber
%\\
%&\leq |\mathcal{A}|e^{-\beta_{t}/2}.
%%
%\end{align}
%%
%To obtain the result in the statement of Lemma \ref{lemma1}, select the constant sequence $\beta_t$ such that $|\mathcal{A}|e^{\beta_{t}/2}=\frac{\delta}{\pi_{t}}$, with scalar parameter sequence $\pi_{t} := \pi^{2}t^{2}/6$. Applying the union bound again over all time points $t \in \mathbb{N}$, we get 
%%
%\begin{align}
%% 
%P\Big\{\bigcup_{t=1}^{\infty}& |f(\bbx)-\hat{\mu}_{t-1}(\bbx)|>\beta_{t}^{1/2}\hat{\sigma}_{t-1}(\bbx)\Big\}\nonumber
%\\
%\leq& \sum_{t=1}^{\infty} P\Big\{|f(\bbx)-\hat{\mu}_{t-1}(\bbx)|>\beta_{t}^{1/2}\hat{\sigma}_{t-1}(\bbx)\Big\}\nonumber\\
%\leq& \sum^{\infty}_{t=1}\frac{\delta}{\pi_{t}}\nonumber\\ 
%=& \delta.
%%
%\end{align}
%%
%The last equality $\sum^{\infty}_{t=1}\frac{\delta}{\pi_{t}} = \delta$ is true since $\sum^{\infty}_{t=1}1/t^{2} = \pi^{2}/6$. 
%We can now change the inequality to obtain an upper bound on the absolute difference between the true function and the estimated mean function for all $\bbx \in \mathcal{A}$ and $t \geq 1$ such that
%\begin{align}
%%
%	|f(\bbx)-\hat{\mu}_{t-1}(\bbx)| \leq {\beta}_{t}^{1/2}\hat{\sigma}_{t-1}(\bbx),\hspace{0.1in} \forall \bbx \in \mathcal{A}, \ \forall t \geq 1
%	%
%\end{align}
%holds with probability $1-\delta$. This completes the proof.
%	\end{proof}
%%%%%%%%%%%%%%%%%%%%%%%%%%%%%%%%%%%%%%%%%%%%%%%%%%%%%%%%%%%%%%%%%%%%%%%%%%%%%%%%%%%%%%%%%%%%%%%%%%%%%%%%%%%%%%%%%%%%%%%%%%%%%%%%%%%%%%%%%%%%%%%%%%%%%L E M M A%%%%%%%%%%%%%%%%%%%%%%%%%%%%%%%%%%%%
%%%%%%%%%%%%%%%%%%%%%%%%%%%%%%%%%%%%%%%%%%%%%%%%%%%%%%%%%%%%%%%%%%%%%%%%%%%%%%%%%%%%%%%%%%%%%%%%%%%%%%%%%%%%%%%%%%%%%%%%%%%%%%%%%%%%%%%%%%%
%
%\begin{lemma}\label{lemma2}
%%
%	Fix $t \geq 1$. If 	$|f(\bbx)-\hat{\mu}_{t-1}(\bbx)| \leq \beta_{t}^{1/2}\hat{\sigma}_{t-1}(\bbx)$ for all $\bbx \in D$, the instantaneous regret is bound as
%	%
%	\begin{align}\label{eq:lemma2}
%	%
%	r_{t} \leq 2\beta_{t}^{1/2}\hat{\sigma}_{t-1}(\bbx_{t})
%	%
%	\end{align}
%	%
%\end{lemma}
%%
%	%%%%%%%%%%%%%%%%%%%%%%%%%%%%%%%%%%%%%%%%%%%%%%%%%%%%%%%%%%%%%%%%%%%%%%%%%%%%%%%%%%%%%%%%%%%%%%%%%%%%%%%%%%%%%%%%%%%%%%%%%%%%%%%%%%%%%%%%%%%%%%%%%%% P  R  O  O  F%%%%%%%%%%%%%%%%%%%%%%%%%%%%%%%%%%%%%%%%%%%%%%%%
%%%%%%%%%%%%%%%%%%%%%%%%%%%%%%%%%%%%%%%%%%%%%%%%%%%%%%%%%%%%%%%%%%%%%%%%%%%%%%%%%%%%%%%%%%%%%%%%%%%%%%%%%%%%%%%%%%%%%%%%%%%%%%%%%%%%%%%%%%%
%	\begin{proof}
%Since the GP-UCB algorithm chooses the next sampling point $\bbx_{t}$ as the argmax of $\hat{\mu}_{t-1}(\bbx)+\sqrt{\beta_{t}}\hat{\sigma}_{t-1}(\bbx)$ at each step, we have
%%
% \begin{align}
%  \hat{\mu}_{t-1}(\hat\bbx_{t})+\sqrt{\beta_{t}}\hat{\sigma}_{t}(\hat\bbx_{t}) &\geq  \hat{\mu}_{t-1}(\bbx^{\star})+\sqrt{\beta_{t}}\hat{\sigma}_{t-1}(\bbx^{\star})\nonumber 
%  \\
%   &\geq f(\bbx^{\star}),
% \end{align} 
% %
%(\red{Need to discuss the above inequality, I am unclear on how we know this upper bounds the optimal even in the origianl paper \citep'{srinivas2012information}. It is coming from unraveling the absolute value in Lemma 1, perhaps?}) where $\bbx^{\star}$ is the optimal point. The instantaneous regret is then bounded as
% %
%\begin{align}
%%
%r_{t} =& f(\bbx^{\star})-f(\hat\bbx_{t}) \nonumber 
%\\
%\leq&  \hat{\mu}_{t-1}(\hat\bbx)+\beta^{1/2}_{t}\hat{\sigma}_{t-1}(\hat\bbx_{t})-f(\hat\bbx_{t}).
%%
%\end{align}
%%
%But from Lemma \ref{lemma1} we have that $|f(\bbx)-\hat{\mu}_{t-1}(\bbx)| \leq \beta_{t}^{1/2}\hat{\sigma}_{t-1}(\bbx)$ holds with probability $1-\delta$. This implies that 
%%\blue{This statement should only hold with high probability. Please clarify. Also what is $1(x^*)$?}, thus we obtain
%%%
%\begin{align}\label{regret1}
%%
%r_{t} = f(\bbx^{\star})-f(\hat\bbx_{t}) \leq  2\sqrt{\beta_{t}}\hat{\sigma}_{t-1}(\hat\bbx_{t}).
%%
%\end{align}
%%
%The expression in \eqref{regret1} represents the regret at instant $t$ for action $\hat{\bbx}_t$ taken by the proposed algorithm. 
%\end{proof}
%%%%%%%%%%%%%%%%%%%%%%%%%%%%%%%%%%%%%%%%%%%%%%%%%%%%%%%%%%%%%%%%%%%%%%%%%%%%%%%%%%%%%%%%%%%%%%%%%%%%%%%%%%%%%%%%%%%%%%%%%%%%%%%%%%%%%%%%%%%%%%%%%%%%%L E M M A%%%%%%%%%%%%%%%%%%%%%%%%%%%%%%%%%%%%
%%%%%%%%%%%%%%%%%%%%%%%%%%%%%%%%%%%%%%%%%%%%%%%%%%%%%%%%%%%%%%%%%%%%%%%%%%%%%%%%%%%%%%%%%%%%%%%%%%%%%%%%%%%%%%%%%%%%%%%%%%%%%%%%%%%%%%%%%%%
%\begin{lemma}\label{lemma3}
%%
%	The information gain for the points selected can be expressed in terms of the predicted variances. If $\bbf_T=(f(\hat\bbx_t))\in\mathbb{R}^T$:
%	%
%	\begin{align}
%	%
%I(\hat\bby_{T};\hat\bbf_{T})=& 
%\frac{1}{2} \sum_{t\in M_T(\epsilon)}\log(1+\sigma^{-2}\hat{\sigma}^{2}_{t-1}(\bbx_{t}))
%%
%	\end{align}
%	where $M_T(\epsilon)$ denotes the number of elements in the dictionary $\bbD_T$ and note that $M_T(0)=T$.
%	%
%\end{lemma}
%%
%	%%%%%%%%%%%%%%%%%%%%%%%%%%%%%%%%%%%%%%%%%%%%%%%%%%%%%%%%%%%%%%%%%%%%%%%%%%%%%%%%%%%%%%%%%%%%%%%%%%%%%%%%%%%%%%%%%%%%%%%%%%%%%%%%%%%%%%%%%%%%%%%%%%% P  R  O  O  F%%%%%%%%%%%%%%%%%%%%%%%%%%%%%%%%%%%%%%%%%%%%%%%%
%%%%%%%%%%%%%%%%%%%%%%%%%%%%%%%%%%%%%%%%%%%%%%%%%%%%%%%%%%%%%%%%%%%%%%%%%%%%%%%%%%%%%%%%%%%%%%%%%%%%%%%%%%%%%%%%%%%%%%%%%%%%%%%%%%%%%%%%%%%
%	\begin{proof}
%	%
%We remark that for the standard GP-UCB algorithm, at each iteration $t$, we have $\bby_t=[y_1, y_2, \cdots, y_t]^T$ which collects all the observations till $t$, and correspondingly in dictionary, we store $\bbX_t=[\bbx_1, \bbx_2, \cdots, \bbx_t]$ which collects all the actions takes so far. But for the compressed CGP-UCB algorithm, since we are only selecting a subset of the elements from $\hat{\bby}_t :=\{\hat y_{i}\}\in \bbD_t$ and $|\bbD_t| \leq t$ for all $t$ due to the $\epsilon$ compression at each step. For a Gaussian with covariance matrix $\sigma^{2}\bbI$, the information gain is~\citep'{cover2012elements} is given by 
%%
%\begin{align}\label{information}
%%
%	I(\bby_{t};\bbf_{t}) = \mathbf{H}(\bby_{t})-\frac{1}{2}\log|2\pi e\sigma^{2}\bbI|,
%	%
%\end{align}
%where it holds that
%\begin{align}\label{first0}
%%
%\frac{1}{2}\log|2\pi e\sigma^{2}\bbI| = \frac{1}{2}\sum^{T}_{t=1}\log(2\pi e\sigma^{2})
%%
%\end{align}
%% In a similar way, we can write 
%Since $\bby_t\in\mathbb{R}^t$. In contrast, for the proposed CGP-UCB algorithm, we have $\hat\bby_t\in\mathbb{R}^{M_t}$ where $M_t(\epsilon)=|\bbD_t|$ represents the model order of the GP posterior distribution. %
%%\begin{align}
%%%
%%	I(\hat\bby_{t};\hat\bbf_{t}) = \mathbf{H}(\hat \bby_{t})-\frac{1}{2}\log|2\pi e\sigma^{2}\bbI|,
%%	%
%%\end{align}
%%where it holds that
%%\begin{align}\label{first}
%%%
%%\frac{1}{2}\log|2\pi e\sigma^{2}\bbI| = \frac{1}{2}\sum^{|\bbD_t|}_{t=1}\log(2\pi e\sigma^{2}).
%%%
%%\end{align}
%%
%Next, by expanding the entropy term $\mathbf{H}(\tilde\bby_{t})$ where $\tilde\bby_{t}=[\hat\bby_{t-1}; \hat y_{t}]$ before the compression,  we can write
%%
%\begin{align}\label{second}
%%
%%
%\mathbf{H}(\hat\bby_{t}) 
%&= \mathbf{H}(\hat\bby_{t-1})+\mathbf{H}(y_{t}|\hat\bby_{t-1}) 
%\\
%&= \mathbf{H}(\hat\bby_{t-1})+\frac{1}{2}\log\big(2\pi e(\sigma^{2}+\hat{\sigma}^{2}_{t-1}(\hat\bbx_{t}))\big). \nonumber
%%
%%&= \frac{1}{2}\sum^{T}_{t=1}\log(2\pi e\sigma^{2})+\frac{1}{2} \sum^{T}_{t=1}\log(1+\sigma^{-2}\hat{\sigma}^{2}_{t-1}(\bbx_{T})).\nonumber
%%
%%
%\end{align}
%We add the current information $\mathbf{H}(y_{t}|\hat\bby_{t-1})$ only if it is more than $\epsilon$ other other wise we don't. This also implies that we drop the update if $|\mathbf{H}(\hat\bby_{t})- \mathbf{H}(\hat\bby_{t-1})| \leq \epsilon$. The above expression holds for each $t$, now take summation over $t=1$ to $T$, since $\bbH(\hat\bby_0)=0$, we get 
%\begin{align}\label{third}
%%
%%
%\mathbf{H}(\hat\bby_{T}) 
%=& \frac{1}{2}\sum_{t\in M_T(\epsilon)}\log(2\pi e\sigma^{2})\nonumber
%\\
%&+\frac{1}{2} \sum_{t\in M_T(\epsilon)}\log(1+\sigma^{-2}\hat{\sigma}^{2}_{t-1}(\hat\bbx_{t})).
%%
%%
%\end{align}
%%
%%Add subtract the term $\frac{1}{2} \sum^{T}_{t=1}\log(1+\sigma^{-2}{\sigma}^{2}_{T-1}(\bbx_{T}))$, we get 
%%\begin{align}\label{third1}
%%%
%%%
%%\mathbf{H}(\hat\bby_{T}) 
%%=& \frac{1}{2}\sum^{T}_{t=1}\log(2\pi e\sigma^{2})+\frac{1}{2} \sum^{T}_{t=1}\log(1+\sigma^{-2}{\sigma}^{2}_{T-1}(\bbx_{T}))\nonumber
%%\\
%%&+\frac{1}{2} \sum^{T}_{t=1}\log\left(\frac{1+\sigma^{-2}\hat{\sigma}^{2}_{T-1}(\bbx_{T})}{1+\sigma^{-2}{\sigma}^{2}_{T-1}(\bbx_{T})}\right).
%%%
%%%
%%\end{align}
%From the update in \eqref{information}, it holds that
%\begin{align}\label{fourth}
%%
%%
%I(\hat\bby_{T};\hat\bbf_{T})=& 
%\frac{1}{2} \sum_{t\in M_T(\epsilon)}\log(1+\sigma^{-2}\hat{\sigma}^{2}_{t-1}(\hat\bbx_{t})).
%%\\
%%&+\frac{1}{2} \sum^{T}_{t=1}\log\left(\frac{1+\sigma^{-2}\hat{\sigma}^{2}_{T-1}(\bbx_{T})}{1+\sigma^{-2}{\sigma}^{2}_{T-1}(\bbx_{T})}\right).
%%%
%%%
%\end{align} 
%%From the expression in \eqref{first} and \eqref{second}, we obtain the information gain expression presented in the statement of Lemma \ref{lemma3}. 
%%At this step, no conclusion can be drawn about the effect of the compression sub-routine on the information gain which depends on the posterior covariance $\hat{\sigma}_{t}(x_{t})$.
%\end{proof}
%%\begin{lemma}
%%	Pick $\delta \in (0,1)$ and let $\beta_{t}$ be defined as in Lemma 1 as $\beta_{t} = \log(|D|t^{2}\pi^{2}/6\delta)$, then with probability $1-\delta$, the following holds
%%%%%%%%%%%%%%%%%%%%%%%%%%%%%%%%%%%%%%%%%%%%%%%%%%%%%%%%%%%%%%%%%%%%%%%%%%%%%%%%%%%%%%%%%%%%%%%%%%%%%%%%%%%%%%%%%%%%%%%%%%%%%%%%%%%%%%%%%%%%%%%%%%%%T H E O R E M%%%%%%%%%%%%%%%%%%%%%%%%%%%%%%%%%%%%
%%%%%%%%%%%%%%%%%%%%%%%%%%%%%%%%%%%%%%%%%%%%%%%%%%%%%%%%%%%%%%%%%%%%%%%%%%%%%%%%%%%%%%%%%%%%%%%%%%%%%%%%%%%%%%%%%%%%%%%%%%%%%%%%%%%%%%%%%%%
%
%For  a finite action space $\mathcal{A}$, we have the following result.
%\begin{theorem}
%For $\delta\in(0,1)$ and $\beta_t=2\log\left(|\mathcal{A}|t^2\pi^2/6\delta\right)$, the sequence of actions $\hat{\bbx_t}$ obtained by the proposed algorithm CGP-UCB achieves the regret bound of $\mathcal{O}^\ast\left(\sqrt{T\gamma_T\log|\mathcal{A}|}+T\sqrt{\epsilon}\right)$ where $\epsilon$ is the compression budget. To be precise, it holds that 
%%
%\begin{align}
%\text{P}\Big\{R_T\leq\sqrt{C_1T\beta_T\gamma_T}+T\sqrt{\epsilon}\ \ \ \forall
%T\geq 1\Big\}\geq 1-\delta
%\end{align}
%where $C_1=\frac{8}{\log\left(1+\sigma^{-2}\right)}$.
%\end{theorem}
%%
%%
%\begin{proof}
%%
%By Lemma \ref{lemma1} and \ref{lemma2}, we have 
%%
%\begin{align}\label{regret}
%r_{t}^{2} \leq 4\beta_{t}\hat{\sigma}_{t-1}^{2}(\hat\bbx_{t})
%\end{align}
%%
% for all $t$ and holds with probability $1-\delta$. Since $\beta_{t}$ is non-decreasing, we obtain
%%
%\begin{align}
%%
%4\beta_{t}\hat{\sigma}_{t-1}^{2}(\hat\bbx_{t}) \leq 4\beta_{T}\sigma^2(\sigma^{-2}\hat{\sigma}_{t-1}^{2}(\hat\bbx_{t})).
%%
%\end{align}
%%
%%\begin{align}
%%%
%%\sum^{T}_{t=1} r_{t}^{2} \leq C_{1}\beta_{T}I(y_{T};f_{T}) \leq C_{1}\beta_{T}y_{T}
%%%
%%	\end{align}
%%	%
%%
%In addition, note that, by definition, we restrict $\kappa(\bbx,\bbx') \leq 1$. Thus, $\hat{\sigma}^{2}_{t-1}(\hat\bbx_{t}) = \kappa(\hat\bbx_{t},\bbx_{t}) \leq 1$ for all $t$. Furthermore, 
%using the fact that $\frac{s}{\log(1+s)}$ is monotonically increasing for positive $s$, we get
%%
%\begin{align}
%%
%\frac{\sigma^{-2}\hat{\sigma}^{2}_{t-1}(\hat\bbx_{t})}{\log(1+\sigma^{-2}\hat{\sigma}^{2}_{t-1}(\hat\bbx_{t}))} \leq \frac{\sigma^{-2}}{\log(1+\sigma^{-2})}.
%%
%\end{align} 
%This implies that
%\begin{align}
%%
%{\sigma^{-2}\hat{\sigma}^{2}_{t-1}(\hat\bbx_{t})} \leq \frac{\sigma^{-2}}{\log(1+\sigma^{-2})}{\log(1+\sigma^{-2}\hat{\sigma}^{2}_{t-1}(\hat\bbx_{t}))}.
%%
%\end{align} 
%%
%Multiplying both sides by $4\beta_{T}\sigma^{2}$, we obtain
%%
%\begin{align}\label{upper_bound}
%%
%4\beta_{T}\hat{\sigma}^{2}_{t-1}(\hat\bbx_{t})%
%\leq 4\beta_{T}C_{2} \log(1+\sigma^{-2}\hat{\sigma}^{2}_{t-1}(\hat\bbx_{t}))
%%
%\end{align}
%%
%where $C_{2} = \frac{\sigma^{-2}}{\log(1+\sigma^{-2})}$. Next, substitute the upper bound in \eqref{upper_bound} on the right hand side of \eqref{regret}, we get 
%%square the both sides and sum over all $t$, we get
%%
%%where $C_{1} = 8/\log(1+\sigma^{-2}) \geq 8\sigma^{2}$ and $\beta_{T}$ is $\beta_{t}$ at $t=T$. Using the lemmas above, we can obtain
%\begin{align}\label{theorem_1}
%%
%%\begin{split}
%%
%\sum^{T}_{t=1}r_{t}^{2} &\leq 4\beta_{T}{\sigma}^{2}C_{2}\sum^{T}_{t=1}\log(1+\sigma^{-2}\hat{\sigma}^{2}_{t-1}(\hat\bbx_{t}))
%\end{align}
%From the result in Lemma \ref{lemma3} and defining $C_1=8\sigma^2C_2$, we can write
%\begin{align}\label{theorem_1_last}
%\sum^{T}_{t=1}r_{t}^{2}&\leq \beta_{T}C_{1}\left[I(\hat\bby_{T};\hat\bbf_{T})+\epsilon(T-M_T(\epsilon))\right]\nonumber\\
%&\leq \beta_{T}C_{1}\left[I(\hat\bby_{T};\hat\bbf_{T})+\epsilon T\right].
%%\\
%%&\leq \beta_{T}C_{1}I(\bby_{T};\bbf_{T}).
%%
%%\end{split}
%%
%\end{align}
%From the Cauchy-Schwartz inequality, it holds that
%\begin{align}\label{theorem_1_last2}
%\sum^{T}_{t=1}r_{t}&\leq \sqrt{T\sum^{T}_{t=1}r_{t}^{2}}\nonumber
%\\
%&\leq \sqrt{\beta_{T}TC_{1}I(\hat\bby_{T};\hat\bbf_{T})}+T\sqrt{\epsilon}.
%%\\
%%&\leq \beta_{T}C_{1}I(\bby_{T};\bbf_{T}).
%%
%%\end{split}
%%
%\end{align}
%\end{proof}
%Note that without compression, we have $\lim_{T\rightarrow\infty} \frac{1}{T}\sum\limits_{t=1}^{T}r_t=0$ and we call it a "no-regret" algorithm, but with the proposed compression, we have $\lim_{T\rightarrow\infty} \frac{1}{T}\sum\limits_{t=1}^{T}r_t=\mathcal{O}(\sqrt{\epsilon})$ which denotes the price to pay to achieve the finite size of the dictionary. 
%
%
%%Next, consider the general case where $D \in \mathbb{R}^{d}$ is any compact and convex set. Note that since we deal with a continuous set, the lemmas considered before will not be directly applicable since they are a function of size of $D$. The regret bounds for this case requires additional assumptions on the kernel function.
%
%%\begin{lemma}
%%	Choose $\delta \in (0,1)$ and let $\beta_{t} = 2\log(|2\pi_{t}/\delta)$, for some $\pi_{t}$ such that $\sum_{t\geq 1} \pi_{t}^{-1} = 1, \pi_{t} >0$. Then
%%	\begin{align}
%%	|f(\bbx)-{t-1}(\bbx)| \leq \beta_{t}^{1/2}\sigma_{t-1}(\bbx)\hspace{0.1in} \forall \bbx \in D, \forall t \geq 1
%%	\end{align}
%%	holds with probability $\geq 1-\delta$.
%%\end{lemma}
%%The proof is similar to the Lemma 1 except we dont have the function of size of $D$ although it is possible to divide $D$ into finite sets. 
%%\begin{lemma}
%%	Pick $\delta \in (0,1)$ and set $\beta_{t} = 2\log(2\pi_{t}/\delta)+4d\log{(dtbr\sqrt{\log(2da/\delta)}}$, where $\sum_{t\geq1}\pi^{-1}_{t} = 1, \pi_{t} >0$.Let $\tau_{t} = dt^{2}br^{2}\sqrt{\log(2da/\delta)}$. Let $[x^{\star}]_{t}$ denote the closest point in $D_{t}$ to $x^{\star}$. Then,
%%	\begin{align}
%%	|f(x^{\star})-{t-1}(|x^{\star}|_{t})\leq \beta^{1/2}_{t}\sigma_{t-1}(|x^{\star}|_{t})+\frac{1}{t^{2}}, \forall t \geq 1
%%	\end{align}
%%\end{lemma}
%
%
%\subsection{General Decision Set} Now, we extend the results of Theorem 1 to the general settings where $\mathcal{A}\subset \mathcal{R}^d$ is a compact set. Before  performing the analysis, we need an additional assumption on the gradient of GP sample paths as follows. 
%%
%\begin{assumption}\label{ass1}
%Let the action space $\mathcal{A}\subset [0,r]^d$ be a convex and compact $d$ dimensional space with $d\in\mathbb{N}$ and $r>0$. With hight probability, the kernel function $\kappa(\bbx,\bbx')$ satisfies the following conditions for GP sample paths $f$ given by 
%%
%\begin{align}
%\text{P}\Big\{\sup_{\bbx\in\mathcal{A}}\Big|\frac{\partial f}{\partial x_j}\Big|>L\Big\}\leq a\exp\left(\frac{-L^2}{b^2}\right)
%\end{align}
%%
%for some constants $a,b>0$.
%
%\end{assumption} The result in Lemma \ref{lemma1} does not hold for infinite action space $\mathcal{A}$. Hence, we first need to state the equivalent result to Lemma \ref{lemma1} for the general case as follows. 
%
%\begin{lemma}\label{lemma4}
%Let $\delta\in(0,1)$ and set $\beta_t=2\log(\pi_t/\delta)$ such that $\sum\limits_{t\geq}\frac{1}{\pi_t}=1,  \pi_t>0$. Then, it holds that
%\begin{align}
%|f(\hat \bbx_t)-\hat\mu_{t-1}|\leq \beta_t^{1/2}\hat\sigma_{t-1}(\hat\bbx_t), \ \ \forall t\geq 1
%\end{align}
%holds with probability $\geq 1-\delta$.
%\end{lemma}
%\begin{proof}
%For a given $t$ and $\bbx\in\mathcal{A}$, the dictionary $\bbD_{t-1}$ elements are deterministic conditioned on the observations $\hat \bby_{t-1}$, which implies that $f(\bbx)\sim\mathcal{N}(\hat\mu_{t-1(\bbx)},\hat{\sigma}^2_{t-1}(\bbx))$. Following the similar steps to the proof of Lemma \ref{lemma1}, it holds that 
%\begin{align}
%%
%P\Big\{|f(\hat\bbx_t)-\hat{\mu}_{t-1}(\hat\bbx_t)|&>\beta_{t}^{1/2}\hat{\sigma}_{t-1}(\hat\bbx_t)\Big\}\leq e^{-\beta_{t}/2}.
%%
%\end{align}
%Since we have $\beta_t=2\log(\pi_t/\delta)$ and utilizing the union bound for $t\in\mathbb{N}$, we get the statement of Lemma \ref{lemma4}.
%\end{proof}
%
%Now, we need to obtain a valid confidence interval on the optimal $\bbx^\star$. Hence, for the analysis purpose, we will consider the discretization $\mathcal{A}_t\subset \mathcal{A}$ and use the cardinality of $\mathcal{A}_t$ at each time instant $t$ in the analysis. Therefore, since after discretization step, the action space is finite, we can repeat the statement of Lemma \ref{lemma1} here by replacing $\mathcal{A}$ by $\mathcal{A}_t$ provided as follows. 
%
%
%\begin{lemma}\label{lemma5}
%%
%	Choose $\delta \in (0,1)$ and let $\beta_{t} = 2\log(|\mathcal{A}_t|\pi_{t}/\delta)$, for some $\pi_{t}$ such that $\sum_{t\geq 1} \pi_{t}^{-1} = 1, \pi_{t} >0$. Then
%	%
%	\begin{align}\label{eq:lemma5}
%	%
%	|f(\bbx)-\hat{\mu}_{t-1}(\bbx)| \leq {\beta}_{t}^{1/2}\hat{\sigma}_{t-1}(\bbx)\hspace{0.1in} \forall \bbx \in \mathcal{A}_t, \forall t \geq 1
%	%
%	\end{align}
%	%
%	holds with probability $\geq 1-\delta$.
%	%
%	\end{lemma}
%	
%Before discussing the confidence bounds for $\bbx\star$, we provide some inequalities which are important for the analysis. From the assumptions and the union bounds, we write that
%%
%\begin{align}
%P\Big\{\forall i, \forall \bbx\in\mathcal{A}, \Big|\frac{\partial f}{\partial x_i}\Big|<L\Big\}\geq 1-da\exp{\left(\frac{-L^2}{b^2}\right)}.
%\end{align}
%%
%which implies that
%%
%\begin{align}\label{lipschitz}
%|f(\bbx)-f(\bbx')|\leq L\|\bbx-\bbx'\|_1
%\end{align}
%%
%for all $\bbx\in\mathcal{A}$ with probability greater than $1-da\exp{\left(\frac{-L^2}{b^2}\right)}$. This will help us obtaining the confidence of $\bbx^\star$.
%
%For the discretization of action space $\mathcal{A}$ with $\mathcal{A}_t$ of size $(\tau_t)^d$ such that
%%
%\begin{align}
%\|\bbx-[\bbx]_t\|_1\leq \frac{rd}{\tau_t}
%\end{align}
%%
%where $[\bbx]_t$ denotes the closest point in $\mathcal{A}_t$ to the original point $\bbx\in\mathcal{A}$.
%%
%\begin{lemma}\label{confidence_xstar}
% Select $\delta\in(0,1)$ and $\beta_t=2\log(2\pi/\delta)+4d\log(dtbr\sqrt{\log(2da/\delta)})$, where $\sum\limits_{t\geq 1}\pi_t^{-1}=1, \pi>0$, and let $\tau_t=dt^2br\sqrt{\log(2da/\delta)}$, then for $[\bbx^\star]_t$ which is the closest point to $\bbx$ in $\mathcal{A}_t$, it holds that 
%\begin{align}
%\vert f(\bbx^{\star})-\hat\mu_{t-1}([\bbx^{\star}]_{t})\vert\leq\beta_{t}^{1/2}\hat\sigma_{t-1}([\bbx^{\star}]_{t})+{{1}\over{t^{2}}}\quad\,\forall t\geq 1
%\end{align}
%with probability $\geq 1-\delta$.
%\end{lemma}
%
%\begin{proof}
%From \eqref{lipschitz}, the Lipschitz continuity of $f$ holds with probability $1-da\exp{\left(\frac{-L^2}{b^2}\right)}$. This implies that
%\begin{align}
%\forall\bbx\in \mathcal{A},\,\vert f(\bbx)-f(\bbx^{\prime})\vert\leq b\sqrt{\log (2da/\delta)}\Vert \bbx-\bbx^{\prime}\Vert_{1}
%\end{align} 
%with probability $1-\delta/2$. Therefore, we can write  
%\begin{align}
%\forall\bbx\in \mathcal{A},\,\vert f(\bbx)-f([\bbx]_{t})\vert\leq rdb\frac{\sqrt{\log (2da/\delta)}}{\tau_t}.
%\end{align} 
%Next, we can select the discretization parameter as $\tau_t=rdb t^2\sqrt{\log (2da/\delta)}$, we obtain
%\begin{align}\label{final}
%\forall\bbx\in \mathcal{A},\,\vert f(\bbx)-f([\bbx]_{t})\vert\leq\frac{1}{t^2}.
%\end{align}
%From the  above analysis, it holds that $|\mathcal{A}_t|=(rdb t^2\sqrt{\log (2da/\delta)})^d$ and the result in \eqref{final} holds for $\bbx^\star$ and $[\bbx^\star]_t$.
%
%To derive the bound inn the statement of Lemma \ref{confidence_xstar}, using the triangle inequality, it holds that
%\begin{align}
%\vert f(\bbx^{\star})-\hat\mu_{t-1}([\bbx^{\star}]_{t})\vert 
%\leq& \vert f(\bbx^{\star})-\hat\mu_{t-1}(\bbx^{\star})\vert\nonumber
%\\
%&+\vert f(\bbx^{\star})-f([\bbx^{\star}]_{t})\vert.\label{bound}
%\end{align}
%Next, the first term on the right hand side of \eqref{bound} is bounded by using $\delta/2$ in the statement of Lemma \ref{lemma5}, and the second term is bounded from the result in \eqref{final}. Hence, it holds that
%\begin{align}
%\vert f(\bbx^{\star})-\hat\mu_{t-1}([\bbx^{\star}]_{t})\vert 
%\leq&\beta_{t}^{1/2}\hat\sigma_{t-1}([\bbx^{\star}]_{t})+{{1}\over{t^{2}}}.\label{bound2}
%\end{align}
%with probability $1-\delta$, which completes the proof. 
%\end{proof}
%Next, we shift focus to prove the regret bound result for the continuous action space. 
%
%\begin{theorem}
%Under Assumption \ref{ass1}, for $\delta\in(0,1)$ and $$\beta_t=2\log(t^2 2\pi^2/(3\delta))+2d\log(^2dbr\sqrt{\log(4da/\delta)}),$$ the sequence of actions $\hat{\bbx_t}$ obtained by the proposed algorithm CGP-UCB achieves the regret bound of $\mathcal{O}^\ast\left(\sqrt{dT\gamma_T}+T\sqrt{\epsilon}\right)$ where $\epsilon$ is the compression budget. To be precise, it holds that 
%%
%\begin{align}
%\text{P}\Big\{R_T\leq\sqrt{C_1T\beta_T\gamma_T}+2+T\sqrt{\epsilon}\ \ \ \forall
%T\geq 1\Big\}\geq 1-\delta
%\end{align}
%where $C_1=\frac{8}{\log\left(1+\sigma^{-2}\right)}$.
%\end{theorem}
%%
%\begin{proof}
%To prover the result, note that from the definition of $\hat{\bbx}_t$, we can write
%\begin{align}\label{theorem_2_0}
%\hat\mu_{t-1}(\hat{\bbx}_{t})+&\beta^{1/2}_t\hat\sigma_{t-1}(\hat\bbx_t)\nonumber
%\\
%\geq& \hat\mu_{t-1}([\bbx^{\star}]_{t})+\beta^{1/2}_t\hat\sigma_{t-1}([\bbx^{\star}]_{t}).
%\end{align}
%Further, from the statement of Lemma \ref{confidence_xstar}, it holds that
% \begin{align}\label{theorem_2_1}
%\hat\mu_{t-1}([\bbx^{\star}]_{t})+\beta^{1/2}_t\hat\sigma_{t-1}([\bbx^{\star}]_{t})+\frac{1}{t^2}\geq f(\bbx^\star). \end{align}
%Note that we have
%\begin{align}\label{theorem_2_2}
%r_t=f(\bbx^\star)-f(\hat{\bbx}_t)
%\end{align}
%Substituting the upper bound in \eqref{theorem_2_1} to \eqref{theorem_2_1}, we get
%\begin{align}\label{theorem_2_3}
%r_t\leq \hat\mu_{t-1}([\bbx^{\star}]_{t})+\beta^{1/2}_t\hat\sigma_{t-1}([\bbx^{\star}]_{t})+\frac{1}{t^2}-f(\hat{\bbx}_t)
%\end{align}
%Utilizing the upper bound in \eqref{theorem_2_0} into \eqref{theorem_2_3}, we obtain
%\begin{align}\label{theorem_2_4}
%r_t\leq \hat\mu_{t-1}(\hat{\bbx}_t)+\beta^{1/2}_t\hat\sigma_{t-1}(\hat{\bbx}_t)-f(\hat{\bbx}_t)+\frac{1}{t^2}
%\end{align}
%Utilizing the result of Lemma \ref{lemma5}, we get
%\begin{align}\label{theorem_2_5}
%r_t\leq 2\beta^{1/2}_t\hat\sigma_{t-1}(\hat{\bbx}_t)+\frac{1}{t^2}
%\end{align}
%with probability $1-\delta$. Take the summation over $t=1$ to $T$, we can write
%\begin{align}\label{theorem_2_6}
%\sum\limits_{t=1}^{T}r_t\leq \sum\limits_{t=1}^{T}2\beta^{1/2}_t\hat\sigma_{t-1}(\hat{\bbx}_t)+\sum\limits_{t=1}^{T}\frac{1}{t^2}.
%\end{align}
% Next, utilizing the similar steps to \eqref{regret} to \eqref{theorem_1_last2}, we can write 
%\begin{align}\label{theorem_1_last3}
%\sum^{T}_{t=1}r_{t}&\leq \sqrt{\beta_{T}TC_{1}I(\hat\bby_{T};\hat\bbf_{T})}+T\sqrt{\epsilon}+\frac{\pi^2}{6}
%%\\
%%&\leq \beta_{T}C_{1}I(\bby_{T};\bbf_{T}).
%%
%%\end{split}
%%
%\end{align}
%where we have used that $\sum\limits_{t}\leq\pi/6$.\end{proof}
%
%
%Next, we provide the result which shows that for a finite $\epsilon>0$, the number of elements in the dictionary $\bbD_T$ becomes finite as $T\rightarrow\infty$.
%\begin{theorem}
%We need to prove that $M_T(\epsilon)\rightarrow M_{\infty}$ as $T\rightarrow \infty$ where $M_{\infty}$ is some constant $M_{\infty}<\infty$. 
%\end{theorem}
%
%\begin{proof}
%
%\blue{We start with the assumption that even without the compression, the total information gain $\lim_{T\rightarrow\infty} I(\bby_T;\bbf_T)\leq I_{\max}$ is upper bounded by some constant $I_{\max}$. } (\red{Please verify the above statement and see if we need to write it in a more rigourous manner. This should be true for finite or compact spaces, since the amount of information in such spaces in compact. But how to formalize that statement? })
%%  Before proving Lemma \ref{theorem_model_order}, we present a lemma which allows us to relate the stopping criterion of our sparsification procedure to a Hilbert subspace distance.
%% %\red{discussion of lemma}
%% %%%%%%%%%%%%%%%%%%%%%%%%%%%%%%%%%%%%%%%%%%%%%%%%%%%%%%%%%%%%%%%
%% %%% L  E  M  M  A  %%%%%%%%%%%%%%%%%
%% %%%%%%%%%%%%%%%%%%%%%%%%%%%%%%%%%%%%%%%%%%%%%%%%%%%%%%%%%%%%%%%
%% %
%% \begin{lemma}\label{lemma_subspace_dist}
%% Define the distance of an arbitrary feature vector $\bbx$ evaluated by the feature transformation $\phi(\bbx) = \kappa(\bbx, \cdot)$ to $\ccalH_{\bbD}=\text{span}\{\kappa(\bbd_t, \cdot) \}_{t=1}^M$, the subspace of the Hilbert space spanned by a dictionary $\bbD$ of size $M$,  as
%% %
%% \begin{align}\label{eq:hilbert_subspace_dist}
%% %
%% \text{dist}( \kappa(\bbx, \cdot) , \ccalH_{\bbD}) 
%% = \min_{f\in\ccalH_{\bbD}} \| \kappa(\bbx, \cdot) - \bbv^T \bbkappa_{\bbD}(\cdot) \|_{\ccalH} \; .
%% %
%% \end{align}
%% %
%% This set distance simplifies to following least-squares projection when $\bbD \in \reals^{p\times M}$ is fixed
%% %
%% \begin{align}\label{eq:hilbert_subspace_dist_ls}
%% \text{dist}( \kappa(\bbx, \cdot) , \ccalH_{\bbD}) 
%% = \Big\|  \kappa(\bbx,\cdot) 
%%   - [\bbK_{\bbD, \bbD}^{-1} \bbkappa_{\bbD}(\bbx)]^T
%%    \bbkappa_{\bbD}(\cdot) \Big\|_{\ccalH} \; .
%% \end{align}
%% %
%% \end{lemma}
%% 
%% 
%% 
%% %%%%%%%%%%%%%%%%%%%%%%%%%%%%%%%%%%%%%%%%%
%% %%%%%%%%%%%%%%%%%%%%%%%%%%%%%%%%%%%%%%%%%
%% %%%%%%%%    P   R   O   O   F    %%%%%%%%%%%%%%%%%%%%%%% 
%% %%%%%%%%%%%%%%%%%%%%%%%%%%%%%%%%%%%%%%%%%
%% %%%%%%%%%%%%%%%%%%%%%%%%%%%%%%%%%%%%%%%%%
%% %\begin{proof} See Appendix 
%% 
%% %We now present our main result, which says that the model order of $f_t$ remains bounded for all $t$, and depends on the conditioning of the problem setting as well as the feature space.
%% 
%% %\subsection{Proof of Lemma \ref{lemma_subspace_dist}}\label{apx_lemma_subspace_dist}
%% %%%%%%%%%%%%%%%%%%%%%%%%%%%%%%%%%%%%%%%%%
%% %%%%%%%%%%%%%%%%%%%%%%%%%%%%%%%%%%%%%%%%%
%% %%%%%%%%    P   R   O   O   F    %%%%%%%%%%%%%%%%%%%%%%% 
%% %%%%%%%%%%%%%%%%%%%%%%%%%%%%%%%%%%%%%%%%%
%% %%%%%%%%%%%%%%%%%%%%%%%%%%%%%%%%%%%%%%%%%
%% \begin{proof}
%% The distance to the subspace $\ccalH_{\bbD}$ is defined as
%% %
%% \begin{align}\label{eq:subspace_dist}
%% %
%% \text{dist}( \kappa(\bbx, \cdot) , \ccalH_{\bbD_t}) 
%% =& \min_{f\in\ccalH_{\bbD}} \| \kappa(\bbx, \cdot) - \bbv^T \bbkappa_{\bbD}(\cdot) \|_{\ccalH}\nonumber\\ 
%% =& \min_{\bbv\in \reals^{M}} \| \kappa(\bbx, \cdot) - \bbv^T \bbkappa_{\bbD}(\cdot) \|_{\ccalH} \; ,
%% %
%% \end{align}
%% %
%% where the first equality comes from the fact that the dictionary $\bbD$ is fixed, so $\bbv\in \reals^M$ is the only free parameter. Now plug in the minimizing weight vector $\tbv^\star=\bbK_{\bbD_t, \bbD_t}^{-1}\bbkappa_{\bbD_t}(\bbx_t)$ into \eqref{eq:subspace_dist} which is obtained in an analogous manner to the logic which yields \eqref{eq:hatparam_update}. Doing so simplifies \eqref{eq:subspace_dist} to the following
%% %
%% \begin{align}\label{eq:subspace_dist2}
%% %
%% \text{dist}(\kappa(\bbx_t, \cdot) , \ccalH_{\bbD_t}) \!=\!  \Big\|  \kappa(\bbx_t,\cdot) 
%%   - [\bbK_{\bbD_t, \bbD_t}^{-1} \bbkappa_{\bbD_t}(\bbx_t)]^T
%%    \bbkappa_{\bbD_t}(\cdot) \Big\|_{\ccalH} \; .
%% %
%% \end{align}
%% %
%% \end{proof}
%% %%%%%%%%%%%%%%%%%%%%%%%%%%%%%%%%%%%%%%
%% %%%%%%%%%%%%%%%%%%%%%%%%%%%%%%%%%%%%%
%% %%%%%%%%%   S  E   C   T   I    O    N    %%%%%%%%%%%%%%%
%% %%%%%%%%%%%%%%%%%%%%%%%%%%%%%%%%%%%%%
%% %%%%%%%%%%%%%%%%%%%%%%%%%%%%%%%%%%%%%
%% \subsection{Proof of Lemma \ref{theorem_model_order}}\label{apx_theorem_model_order}
% %%%%%%%%%%%%%%%%%%%%%%%%%%%%%%%%%%%%%%%%%
% %%%%%%%%%%%%%%%%%%%%%%%%%%%%%%%%%%%%%%%%%
% %%%%%%%%    P   R   O   O   F    %%%%%%%%%%%%%%%%%%%%%%% 
% %%%%%%%%%%%%%%%%%%%%%%%%%%%%%%%%%%%%%%%%%
% %%%%%%%%%%%%%%%%%%%%%%%%%%%%%%%%%%%%%%%%%
% %\begin{proof}
% %
%Consider the model order of the dictionary $\bbD_{t-1}$ at $t-1$ and $\bbD_{t}$ generated by Algorithm \ref{alg:compressed} denoted by $M_{t-1}$ and $M_{t}$, respectively, at two arbitrary subsequent times $t-1$ and $t$. The number of elements in $\bbD_{t-1}$ are $M_{t-1}=(t-1)$. After performing the algorithm update at $t$, we add a new data points to the dictionary and increase the model order by one, hence $M_{t}=M_{t-1}+1$. Hence, there are only two possibilities, wither we increase $M_{t-1}$ by $1$ at $t$ or not which means $M_{t}=M_{t-1}$.
% %
%% Specifically, rather than allowing the dimension of the Hilbert subspace to which $f$ belongs to grow by $1$ at each time as in \eqref{eq:param_update}, we propose to project them onto time-varying subspaces generated by dictionaries $\bbD=\bbD_{t+1}$ extracted from the data points observed thus far.
% 
%%   Begin by assuming function ${f}_{t+1}$ is parameterized by dictionary $\bbD_{t+1}$ and weight vector $\bbw_{t+1}$. Moreover, we denote columns of $\bbD_{t+1}$ as $\bbd_t$ for $t=1,\dots,{M}_{t+1}$.
% %
% % Assume a constant algorithm step-size $\eta$ has been chosen such that $\eta<1/\lambda$ and the approximation budget $\eps$ satisfies $\eps=K \eta^{3/2}$ for some positive scalar $K>0$.
% %
% Suppose the model order $M_{t}$ is equal to that of $M_{t-1}$, i.e. $M_{t} = M_{t-1}$. This relation holds when $\mathbf{H}(y_{t}|\hat\bby_{t-1}) > \eps$, \emph{is not} satisfied for the new information with the newest data point $y_t$.
% %
% Thus, the negation holds for this case, stated as
% %
% \begin{align}\label{eq:komp_to_terminate}
% \mathbf{H}(y_{t}|\hat\bby_{t-1})  \leq \eps \; .
% \end{align}
% %
% We can write the above equation equivalently as 
%  \begin{align}\label{eq:komp_to_terminate2}
%   \mathbf{H}(\hat \bby_{t})-\mathbf{H}(\hat \bby_{t-1})  \leq \eps \; 
%   \end{align}
%   which describes that we don't update the dictionary if the addition to information gain is less than $\epsilon$. 
%     
%  %Consequently, if $\mathbf{H}(y_{t}|\hat\bby_{t-1})$, then \eqref{eq:komp_to_terminate} holds and the model order does not grow. Thus it suffices to consider $\mathbf{H}(y_{t}|\hat\bby_{t-1})$.
% 
%  
% 
% Now, let's take the contrapositive of the preceding expressions to observe that growth in the model order ($M_{t} = M_{t-1} + 1$) implies that the condition
% %
% \begin{align}
%  \label{eq:min_gamma2}
%  \mathbf{H}(\hat \bby_{t})-\mathbf{H}(\hat \bby_{t-1}) > \epsilon
%  \end{align} %\vspace{-5cm}
% %we only update the
%% which implies that the model order is increased by one only if the information of $\hat \bby_{t}$ is atleast more than the previous point $\hat \bby_{t-1}$ by $\epsilon$.    
%% holds. The above expression implies that 
%% \begin{align}
%% 1-{\boldsymbol{\kappa}}_{{{\bbD}}_{t-1}}(\hat\bbx_{t})^T(\bbK_{t-1}+\sigma^{2}\bbI)^{-1}{\boldsymbol{\kappa}}_{{{\bbD}}_{t-1}}(\hat\bbx_{t})> \frac{\exp(2\epsilon)}{2\pi e}-\sigma^{2}
%% \end{align}
%% 
%% 
%%  Therefore, each time a new point is added to the model, the corresponding kernel function is guaranteed to be at least a distance of {$\frac{\epsilon}{\eta|\check L_t'({f}_t(\bbx_t)) |}$} from every other kernel function in the current model. 
%% 
%% 
%% By the $C$-Lipschitz continuity of the instantaneous loss (Assumption \ref{as:2}): specifically {$1/|\nabla_f \check{L}_t (f_{t}(\bbS_t))| \geq 1/HC$}, we can lower-bound the threshold condition in \eqref{eq:min_gamma2} as 
%% %
%% \begin{align}\label{eq:min_gamma3}
%%  %
%%   \frac{\epsilon}{\eta|\check\ell_t'({f}_t(\bbx_t)) |}\geq \frac{\epsilon}{\eta CH}
%%   %
%%  \end{align}
%% %
%% We have
%%  \begin{align}
%%  \label{eq:min_gamma321}
%%  \text{dist}(\kappa(\bbx_t,\cdot),\ccalH_{\bbD_t}) > \frac{\epsilon}{\eta CH}
%%  \end{align}
%%  %
%% Therefore, For a fixed compression budget $\epsilon$ and step size $\eta$, the KOMP stopping criterion is violated for the newest point whenever distinct dictionary points $\bbd_k$ and $\bbd_j$  for $j,k\in\{1,\dots,M_t\}$, satisfy the condition $\|\phi(\bbd_j) - \phi(\bbd_k) \|_\mathcal{H} > \frac{\epsilon}{\eta CH}$.
% Next, we follow the similar argument as provided in the proof of Theorem 3.1 in \citep'{1315946}.   Since the space $\ccalI:=[0,I_{\max}]\subset \mathbb{R}$ is compact, therefore the number minimum of balls (covering number) of radius $\epsilon$ needed to cover the set $\mathcal{I}$ is finite (see, e.g., \citep'{anthony2009neural}) for a fixed compression budget $\epsilon$.
% 
% % Further for the non-stationary settings, we select the compression budget $\epsilon$ to be inversely proportional to $T$ in order to make regret sublinear, which implies that the radius of $\delta$ balls is going to zero with $T$. Hence, the covering number approaches infinite. Under this condition, it becomes important to study the rate at which the size of the dictionary increases with respect to decrease in the compression budget. 
%%  We can even characterize the rate of model order of the dictionary. Note that from \citep'[Proposition 2.2]{1315946}, it holds for  the number of elements in dictionary that  %\blue{Really interesting... this result is definitely missing from the literature: exactly relating model complexity to compression budget/step-size selection is really interesting. That we have to better accentuate in the {\bf Contribution} discussion in Sec. \ref{sec:Problem}. }
%%  %
%%  \begin{align}\label{model_order_1}
%%  %
%%  M_t\leq \mathcal{O}\left(\frac{1}{\epsilon}\right).
%%  %
%%  \end{align}
%%  %
%% where $Y$ is a constant depends upon $\mathcal{X}$ and the kernel function. By \eqref{eq:min_gamma321}, we have that $\nu=\frac{\epsilon}{\eta CH}$, which we may substitute into \eqref{model_order_1} to obtain
%%  %
%%  \begin{align}\label{model_order_2}
%%  %
%%   M\leq Y(CH)^p\left(\frac{\eta}{\epsilon}\right)^p.
%%   %
%%   \end{align}
%%   %
%%   as stated in \eqref{model_order_0}. The lower bound $H$ in \eqref{model_order_0} comes from the fact that to represent the instantaneous gradient of the windowed loss of length $H$, a minimum of $H$ points are required.  \hfill %  Then, the model order of the learned function will depend on the ratio of the step-size to the compression budget, problem constants such as Lipschitz continuity modulus and the parsimony constant.
%%  % From the above expression, we will get different upper bounds for the different decrement rate of the compression budget  which we will choose in accordance with to minimize the regret. The result in \eqref{model_order_1} holds directly for POLK and related the tradeoff between stepsize and compression budget for POLK. This result was missing from POLK. 
% %
% %\end{proof}
%\end{proof}
%
\subsection{Bound on the Information Gain}

The information gain function $\gamma_T:=I(\hat\bby_{T};\hat\bbf_{T})$ is submodular function, so we can use the greedy maximization to upper bound $\gamma_T$. For $T$, we consider the discretization $\mathcal{A}_T\subset\mathcal{A}$ with $n_T=|\mathcal{A}_T|=T^\tau$ with the nearest neighbor distance of $o(1)$. For the discretized action space $\mathcal{A}_T$, let us consider the kernel matrix $\bbK_{\mathcal{A}_T}\in\mathbb{R}^{n_T\times n_T}$, and we try to bound $\gamma_T$ yb an expression involving the eigen values of the kernel matrix $\bbK_{\mathcal{A}_T}$ denoted by $\{\hat\lambda_t\}$. 
 
 \red{I need to discuss whether to keep this section in the paper or not. I felt like the proof is independent of the compression technique, but I am including here for the completion.  }
\subsubsection{Greedy Maximization and Discretization} For this section, we fix $T\in\mathbb{N}$ and assumes the existence of a discretization $\mathcal{A}_T\subset\mathcal{A}$, with $n_T=|\mathcal{A}_T|$ of the order of $T^\tau$ such that
%
\begin{align}\label{discretization}
\forall \bbx\in\mathcal{A}, \ \ \exists [\bbx]_T\in\mathcal{A}_T\ \ :\ \ \|\bbx-[\bbx]_T\|=\mathcal{O}(T^{\frac{-\tau}{d}}).
\end{align}
%
In this analysis, the information gain is restricted to the subsets $A\subset\mathcal{A}_T$ defined as
%
\begin{align}\label{opt_probelm}
\tilde\gamma_T:=\max_{A\subset\mathcal{A}_T, \ |A|=T} I(\bby_A; \bbf_A).
\end{align}
%
Note that $\tilde\gamma_T\leq \gamma_T$, but we first bound $\tilde\gamma_T$ and later could bound the slack.
%
\begin{lemma}\label{lemma7}
Under Assumption \ref{ass1}, information gain $F(\cdot)$ defined as $F(\{\bbx_t\}_{\forall t})=\frac{1}{2}\log |\bbI+\sigma^{-2}\bbK_{\{\bbx_t\}}|$ is uniformly Lipschitz continuous in each component $\bbx_t\in\mathcal{A}$. 
\end{lemma}
\begin{proof}
From the Assumption \ref{ass1}, it holds that the kernel function $\kappa(\bbx,\bbx')$ is continuously differentiable. Hence, the statement of Lemma \ref{lemma7} holds due to the fact that the information gain function $F(\{\bbx_t\}_{\forall t})$ is continuously differentiable in the kernel matrix $\bbK_{\{\bbx_t\}}$. 
\end{proof}

\begin{lemma}[Bounding the slack]\label{label8}
Let us consider a discretization $\mathcal{A}_T$ such that the conditions in \eqref{discretization} is satisfied, then under the Assumption \ref{ass1}, it holds that
%
\begin{align}
0\leq \gamma_T-\tilde{\gamma}_T=\mathcal{O}(T^{1-\frac{\tau}{d}})
\end{align}
%
\end{lemma}

\begin{proof}
Let us consider the set of actions $A_T=\{\bbx_1,\cdots,\bbx_T\}$ is the solution to the optimization problem in \eqref{opt_probelm} and attains the maximum $\gamma_T$. Let us denote the corresponding discrete version of actions $[A_T]=\{[\bbx_t]_T\}$ which belongs to set $\mathcal{A}_T$. From the definition of $\tilde{\gamma}_T$, we can write
%
\begin{align}
0\leq {\gamma}_T-\tilde{\gamma}_T \leq& {\gamma}_T-I(\bby_{[A_T]}; \bbf_{[A_T]})\nonumber
\\
=& F_T(A)-F_T([A_T])
\end{align}
where we have $F_T([A_T])=\frac{1}{2}\log |\bbI+\sigma^{-2}\bbK_{\{\bbx_t\}}|$. Using the Lipschitz continuous property of $F_A$ from Lemma \ref{lemma7}, it holds that
%
\begin{align}\label{last}
|{\gamma}_T-I(\bby_{[A_T]}; \bbf_{[A_T]})|\leq & \mathcal{O}(T \max_t \|\bbx_t-[\bbx_t]_T\|)\nonumber 
\\
=&\mathcal{O}(T^{1-\frac{\tau}{d}}).
\end{align}
The last equality in \eqref{discretization} holds from the statement in \eqref{discretization}.
\end{proof}

In the rest of the analysis, we focus on bounding the term $\tilde{\gamma}_T$ only because we can  bound the slack as in Lemma \ref{label8}. Let us denote $\bbK_{\mathcal{A}_T}=[\kappa(\bbx,\bbx')]_{\bbx,\bbx'\in\mathcal{A}_T}$ as the kernel matrix for the discretized version $\mathcal{A}_T$ of the action space $\mathcal{A}$. Further, we denote the eigen value decomposition of the kernel matrix as $\bbK_{\mathcal{A}_T}=\bbU\hat{\boldsymbol{\Lambda}}\bbU^T$ where $\hat{\boldsymbol{\Lambda}}$ contains the eigen values $\{\hat{\lambda_t}\}$ such that $\hat{\lambda_1}\geq \hat{\lambda_2}\geq\cdots\geq \hat{\lambda_t}0$ and $\bbU=[\bbu_1, \bbu_2,\cdots]$ collects the orthonormal corresponding eigen vectors.  We remark that if the number of actions in $\mathcal{A}_T$ is less than $T$ which means $n_T<T$, then $\hat{\lambda_t}=0$ for $t=n_T+1$ to $T$


\begin{lemma}
For any $T\geq 1$, the information gain $\tilde\gamma_T$ is upper bounded as 
%
\begin{align}
\tilde{\gamma}_T\leq \frac{1/2}{1-e^{-1}} \max_{m_1,\cdots,m_T} \sum\limits_{t=1}^{T}\log(1+\sigma^{-2}m_t\hat{\lambda}_t)
\end{align}
%
where $m_t\in\mathbb{N}$, $\sum\limits_{t}m_t=T$, where $\hat{\lambda_1}\geq\hat{\lambda_2}\geq\cdots$
\end{lemma}

\begin{proof}

\end{proof}
